# Supplementary material for: Active Screening for Recurrent Diseases: A Reinforcement Learning Approach
Source: arXiv:2101.02766 source file (2021-04-19)
Supplement: Supplementary file 1 [file Appendix.tex]

\section{Belief Update}\label{app:belief}
Our belief update procedure follows that of~\cite{ou2020}.
Let $b^{v}_{t}$ denote the probability of node $v$ being $I$ at time step $t$. Before any observation and action happens, we initialize $b^{v}_{0}=0.5$. Suppose the belief of the probabilities in previous time step \textit{before observation} is $b^{v}_{t-1}$. When the observation is received, the belief of probabilities of the previous time step is then:
\begin{align*}
\hat{b}^{v}_{t-1}=\begin{cases}
1, & v \in \mathbf{o}_t \\
\frac{(1-\gamma)b^{v}_{t-1}}{(1-b^{v}_{t-1})+(1-\gamma)b^{v}_{t-1}}, & otherwise\\
\end{cases}
\end{align*}
%We will show how to obtain, update and encode such probability for the current time step. 

Based on these probabilities, the probability of $v$ being $I$ in the current time step is given by:
\begin{equation}
b^{v}_{t}=\begin{cases}
0, & v \in \mathbf{o}_t, \\
(1-\prod_{u\in \delta(v)} (1-\beta \hat{b}^{u}_{t-1})) (1-\hat{b}^{v}_{t-1})+ \hat{b}^{v}_{t-1} , & otherwise\\
\end{cases}
\end{equation}
in which $\delta(v)$ denotes neighbor of node $v$. Such probability is embed into the GCN of both primary agent and secondary agent $0$, encoded as $\mathbf{s}^{II}_{0}=\mathbf{s}^{I}$. Based on the output of its $Q$ function, each worker $i$ will select its action $a^{II}_{i}$ and add it to the master action set $\mathbf{a}^{I}$. After updating the current belief base on the selected action ($b^{v}_{t}=0$) for $v\in \mathbf{a}^{I}$, $b^{v}_{t}$ will be passed to and encoded by the GCN of next worker as $\mathbf{s}^{II}_{i+1}$. This process repeats until the last worker agent is reached. The final $b^{v}_{t}$ is then used in the belief update of next time step.

\section{Table of Notations}\label{app:notation}
Table~\ref{notation} shows a summary of the notations used in this paper. Note that for simplicity, we do not distinguish between the primary and secondary agents for concepts related to the algorithm.

\begin{table}[ht!]
\caption{Notations for major concepts. }\label{notation}
\setlength\extrarowheight{1pt}
\scalebox{1}{
\begin{tabular}{|c|l|}
\hline
\textbf{Symbol}                & \textbf{Description}              \\ \hline
$G$         & contact network              \\ 
$S$         & susceptible state     \\ 
$I$         & infectious state         \\ 
$\beta$    & transmission probability     \\ 
$\gamma$         & cure probability              \\ 
$t$         & time step \\ 
$T$         & time horizon          \\ 
$k$         & screening budget for each time step  \\ 
$\mathbf{x}_t$    & true state at time $t$ (not available in testing)\\ 
$\mathbf{a}_t$ & set of nodes actively screened (action at time $t$) \\ 
$\mathbf{o}_t$ & set of self-report nodes (observation at time $t$)  \\ 
$\mathbf{b}_t$ & Belief state at time $t$\\%approximate probabilities of each node being in $I$ state    \\ %&\hp{what do you mean by ``marginal"? It appears in Section 4 but not defined anywhere in the paper.}\\
$\mathbf{s}_t$ & state representation for Q function \\
$r_t$ & step wise reward\\
$Q$ & Q function\\
$\alpha$ & future discount factor \\
$\tau$ & auxiliary coefficient for curriculum learning \\
$\bar{r}_t$ & Initial step wise reward for curriculum learning \\
\hline

\end{tabular}
}

\end{table} 
\section{Ablation Study}\label{app:ablation}
To show the effectiveness of our two-level RL framework and the curriculum learning component, we conduct an ablation study on a sample network Face-to-face.
Fig.~\ref{fig:ablation} shows the ablation study results on the Face-to-face network. We evaluate 4 settings:
(i) Single agent without curriculum learning (CL); (ii) Two-level ($k$ agents) RL without CL; (iii) Single agent with CL and (iv) Full (i.e., two-level RL with CL). Note that in (i) and (iii), the remaining budget is directly hard-coded as part of the state information to the GCN.
By comparing (i) with (iii) or comparing (ii) with (iv), we can see that curriculum learning is critical in improving the solution quality. On the other hand, by comparing (i) with (ii) or comparing (iii) with (iv), we can see that the two-level primary and secondary agents framework, which trains a different secondary agent policy, is also improving the solution quality by a large margin. On the contrary, hard-coding the remaining budget into the state leads to sub-optimal solution quality.
\begin{figure}[ht!]
\includegraphics[width=0.47\textwidth,keepaspectratio]{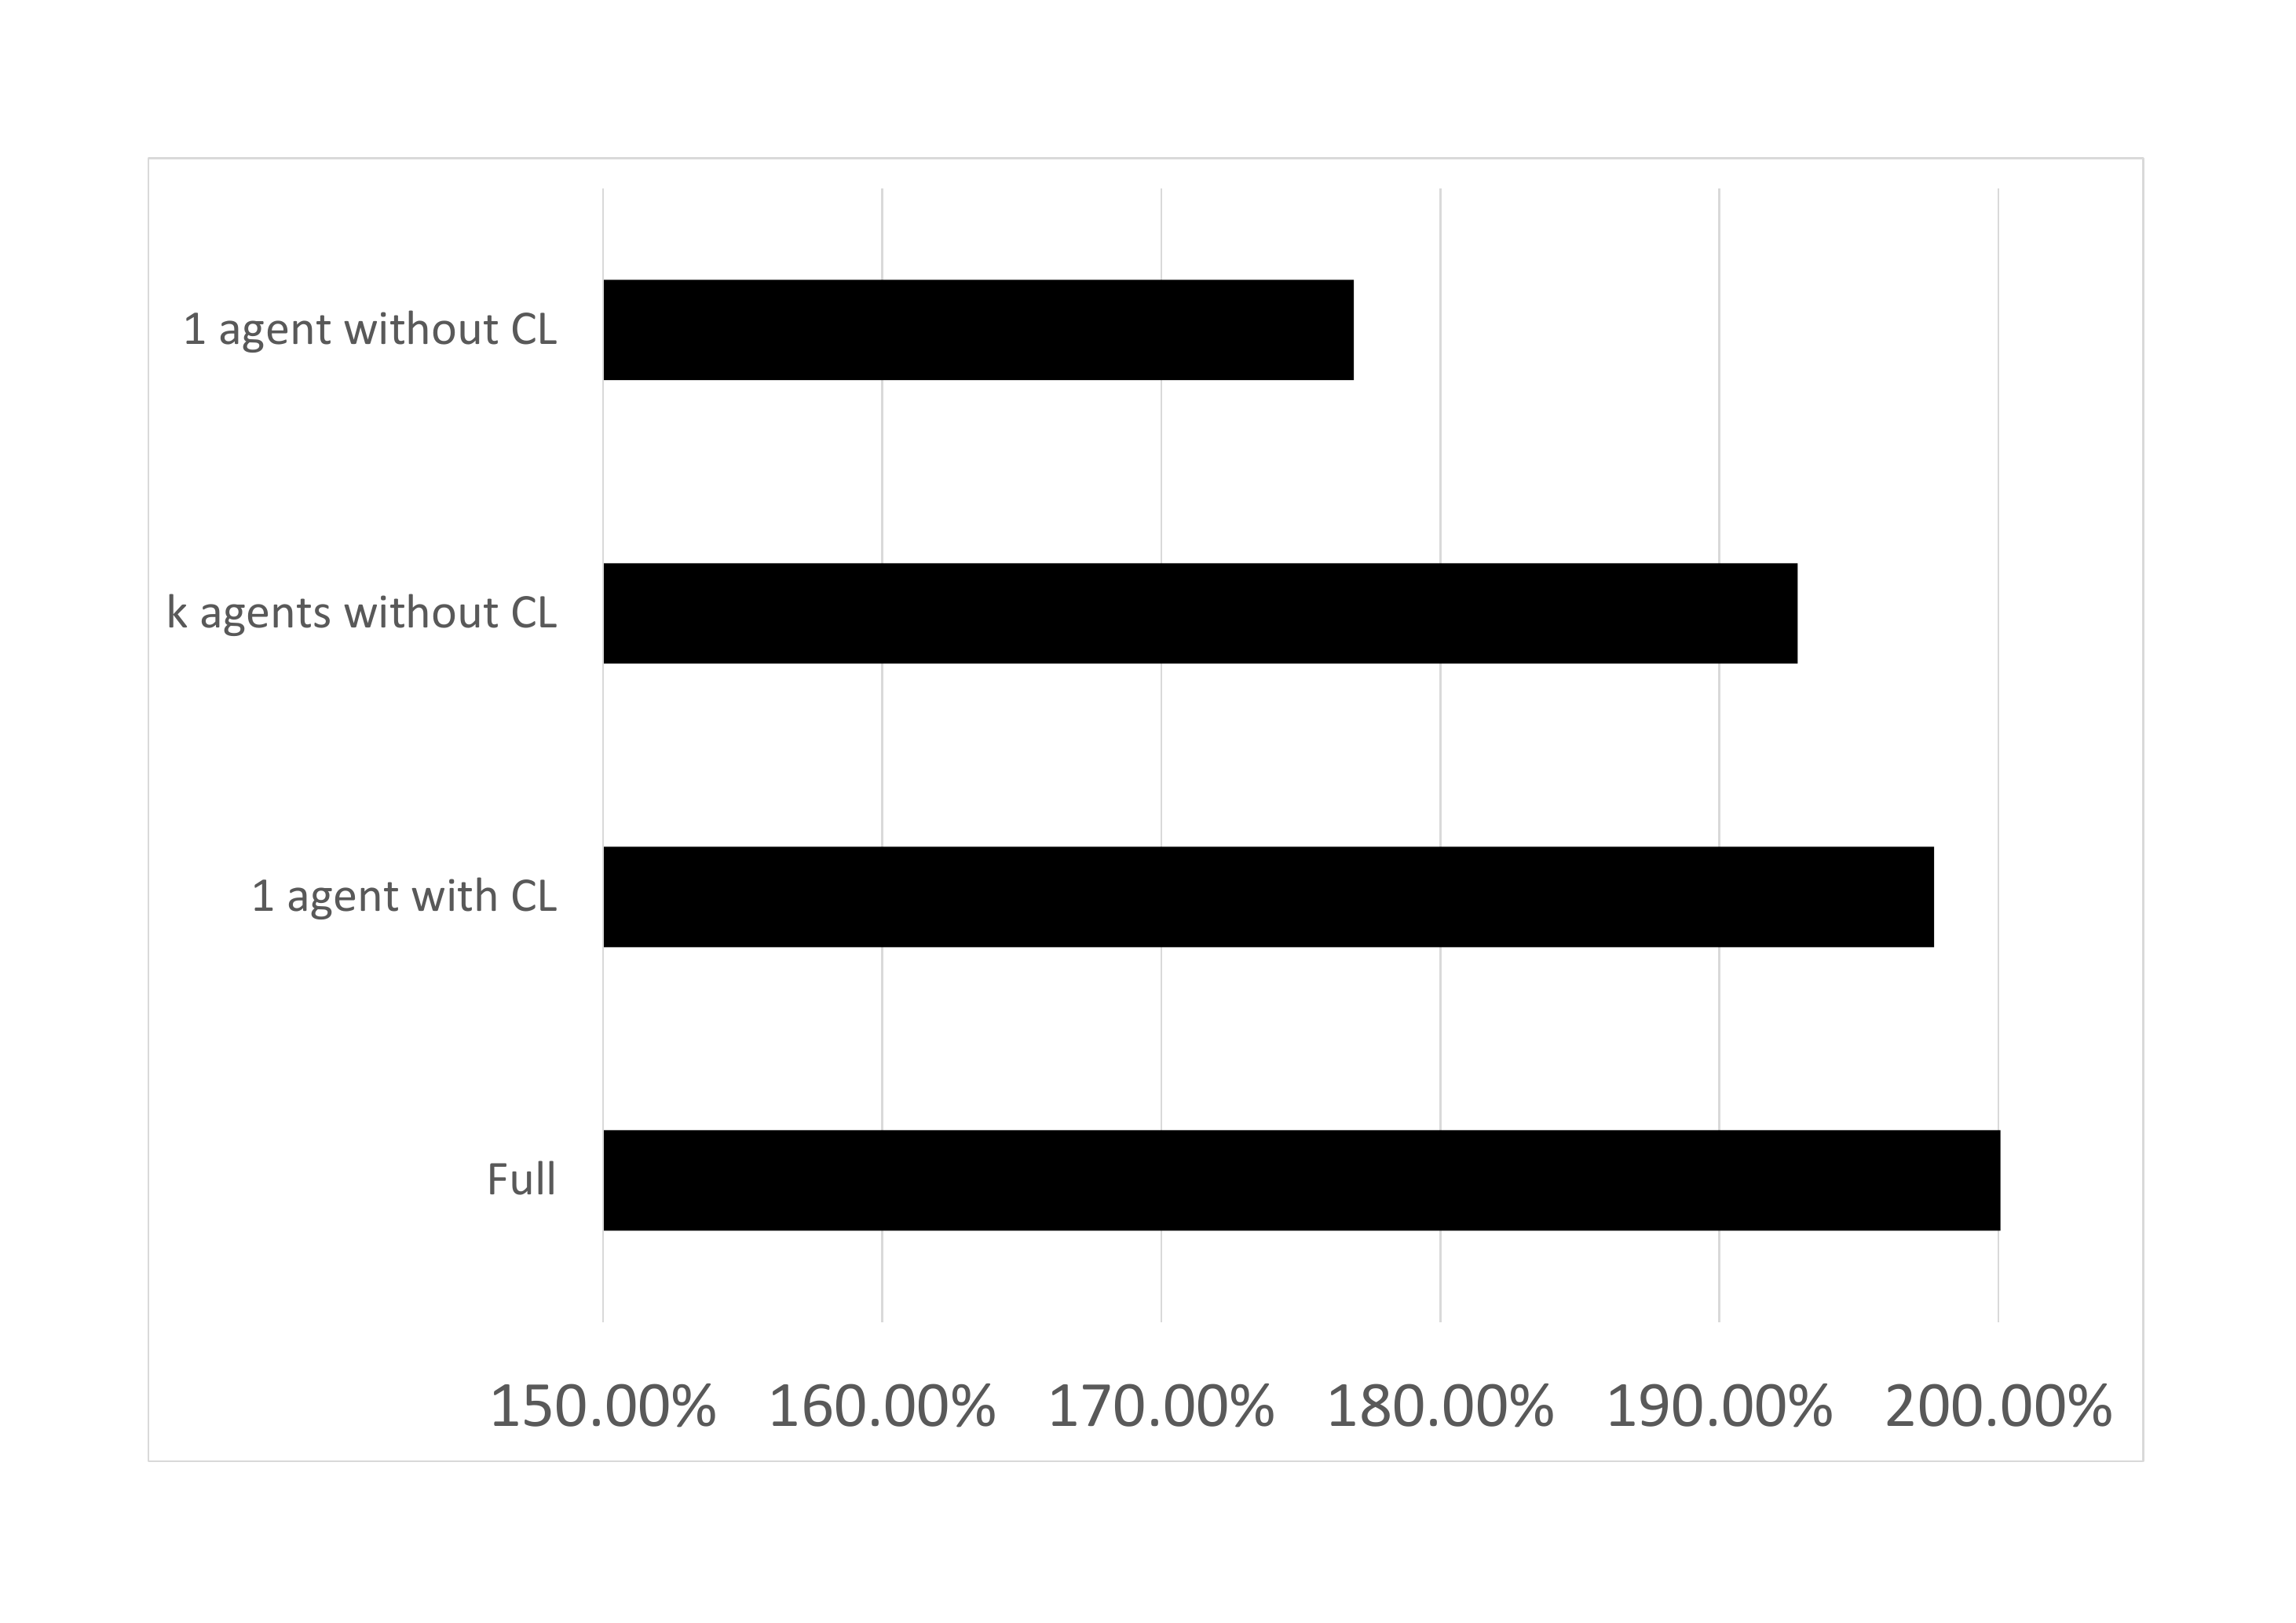}%
\centering
\caption{Ablation study run on the Face-to-face network. The x-axis is the percentage of improvement over no-intervention. The y-axis denotes different variants of our approach.
}\label{fig:ablation}
\end{figure}

\section{Experimental Results on Other Networks}\label{app:exp}
Figure~\ref{timev} to~\ref{node} show subtracted result experiment results of \textit{Hospital}, \textit{India}, \textit{Flu} and \textit{Irvine} network. Similar trends can be observed as in the main text.

\begin{figure*}[t]
\centering
\subfloat[Hospital]{%
  \includegraphics[width=0.35\textwidth,keepaspectratio]{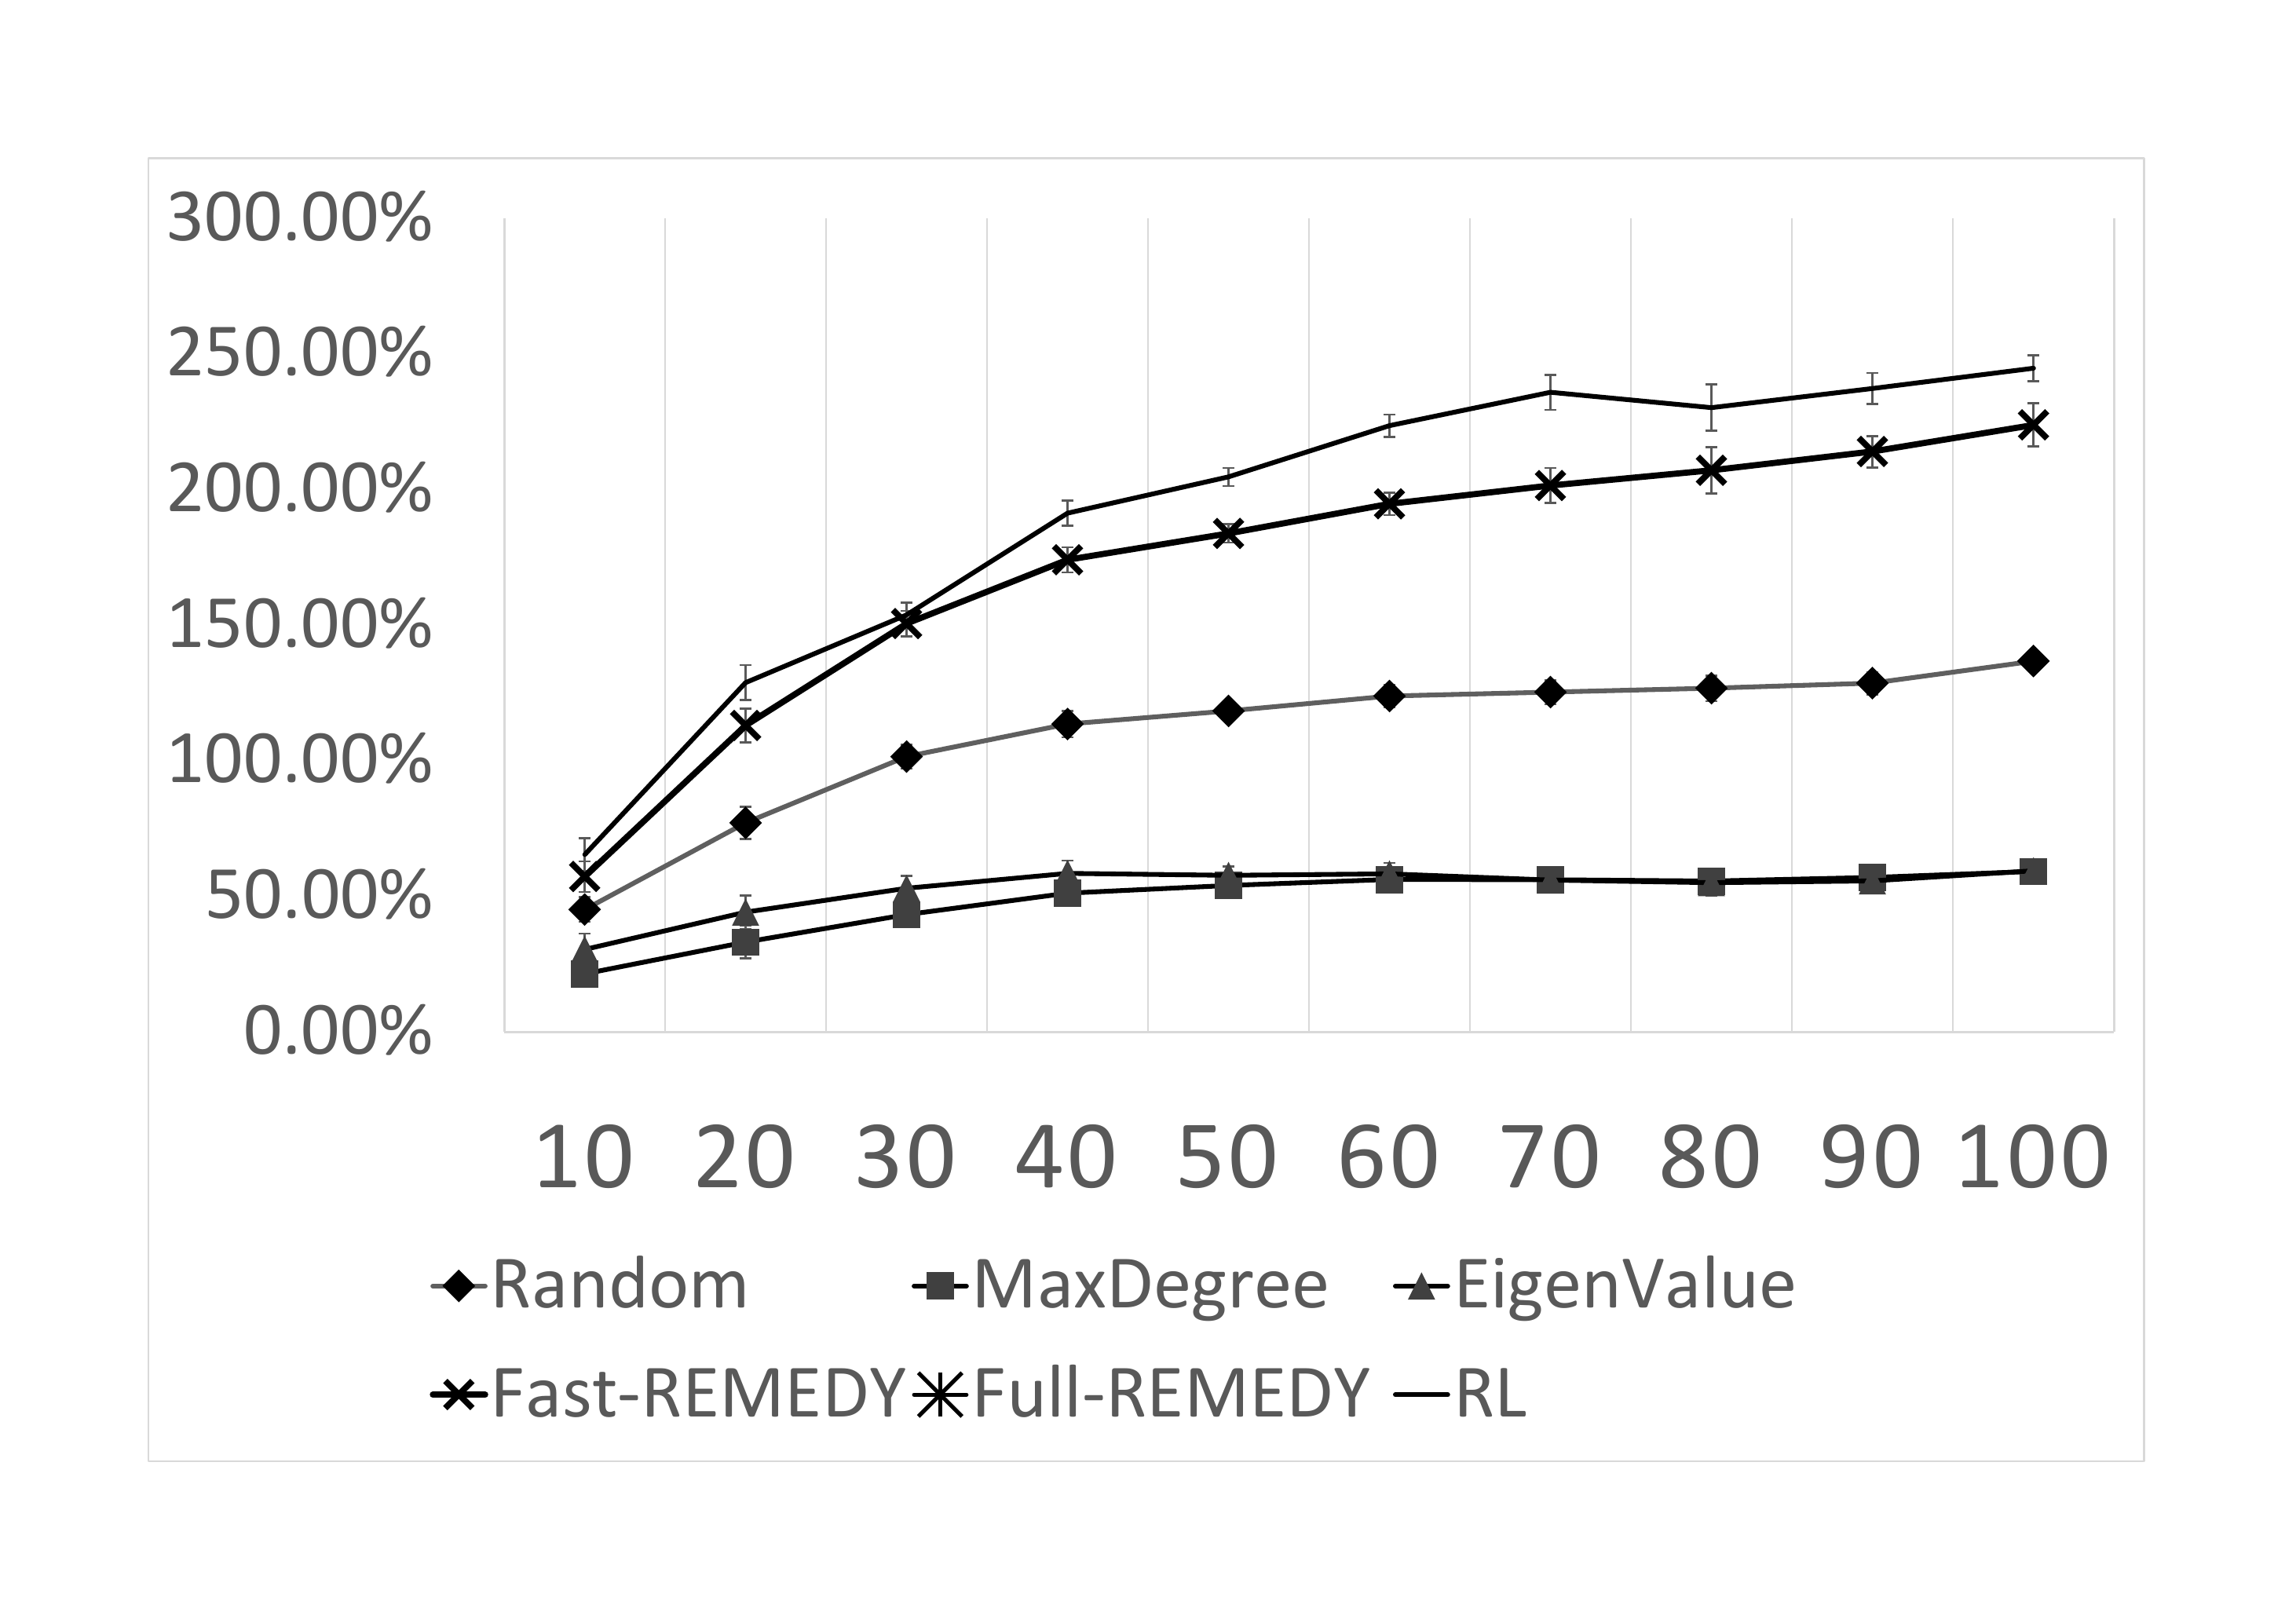}%
}\hfill
\subfloat[India]{%
  \includegraphics[width=0.35\textwidth,keepaspectratio]{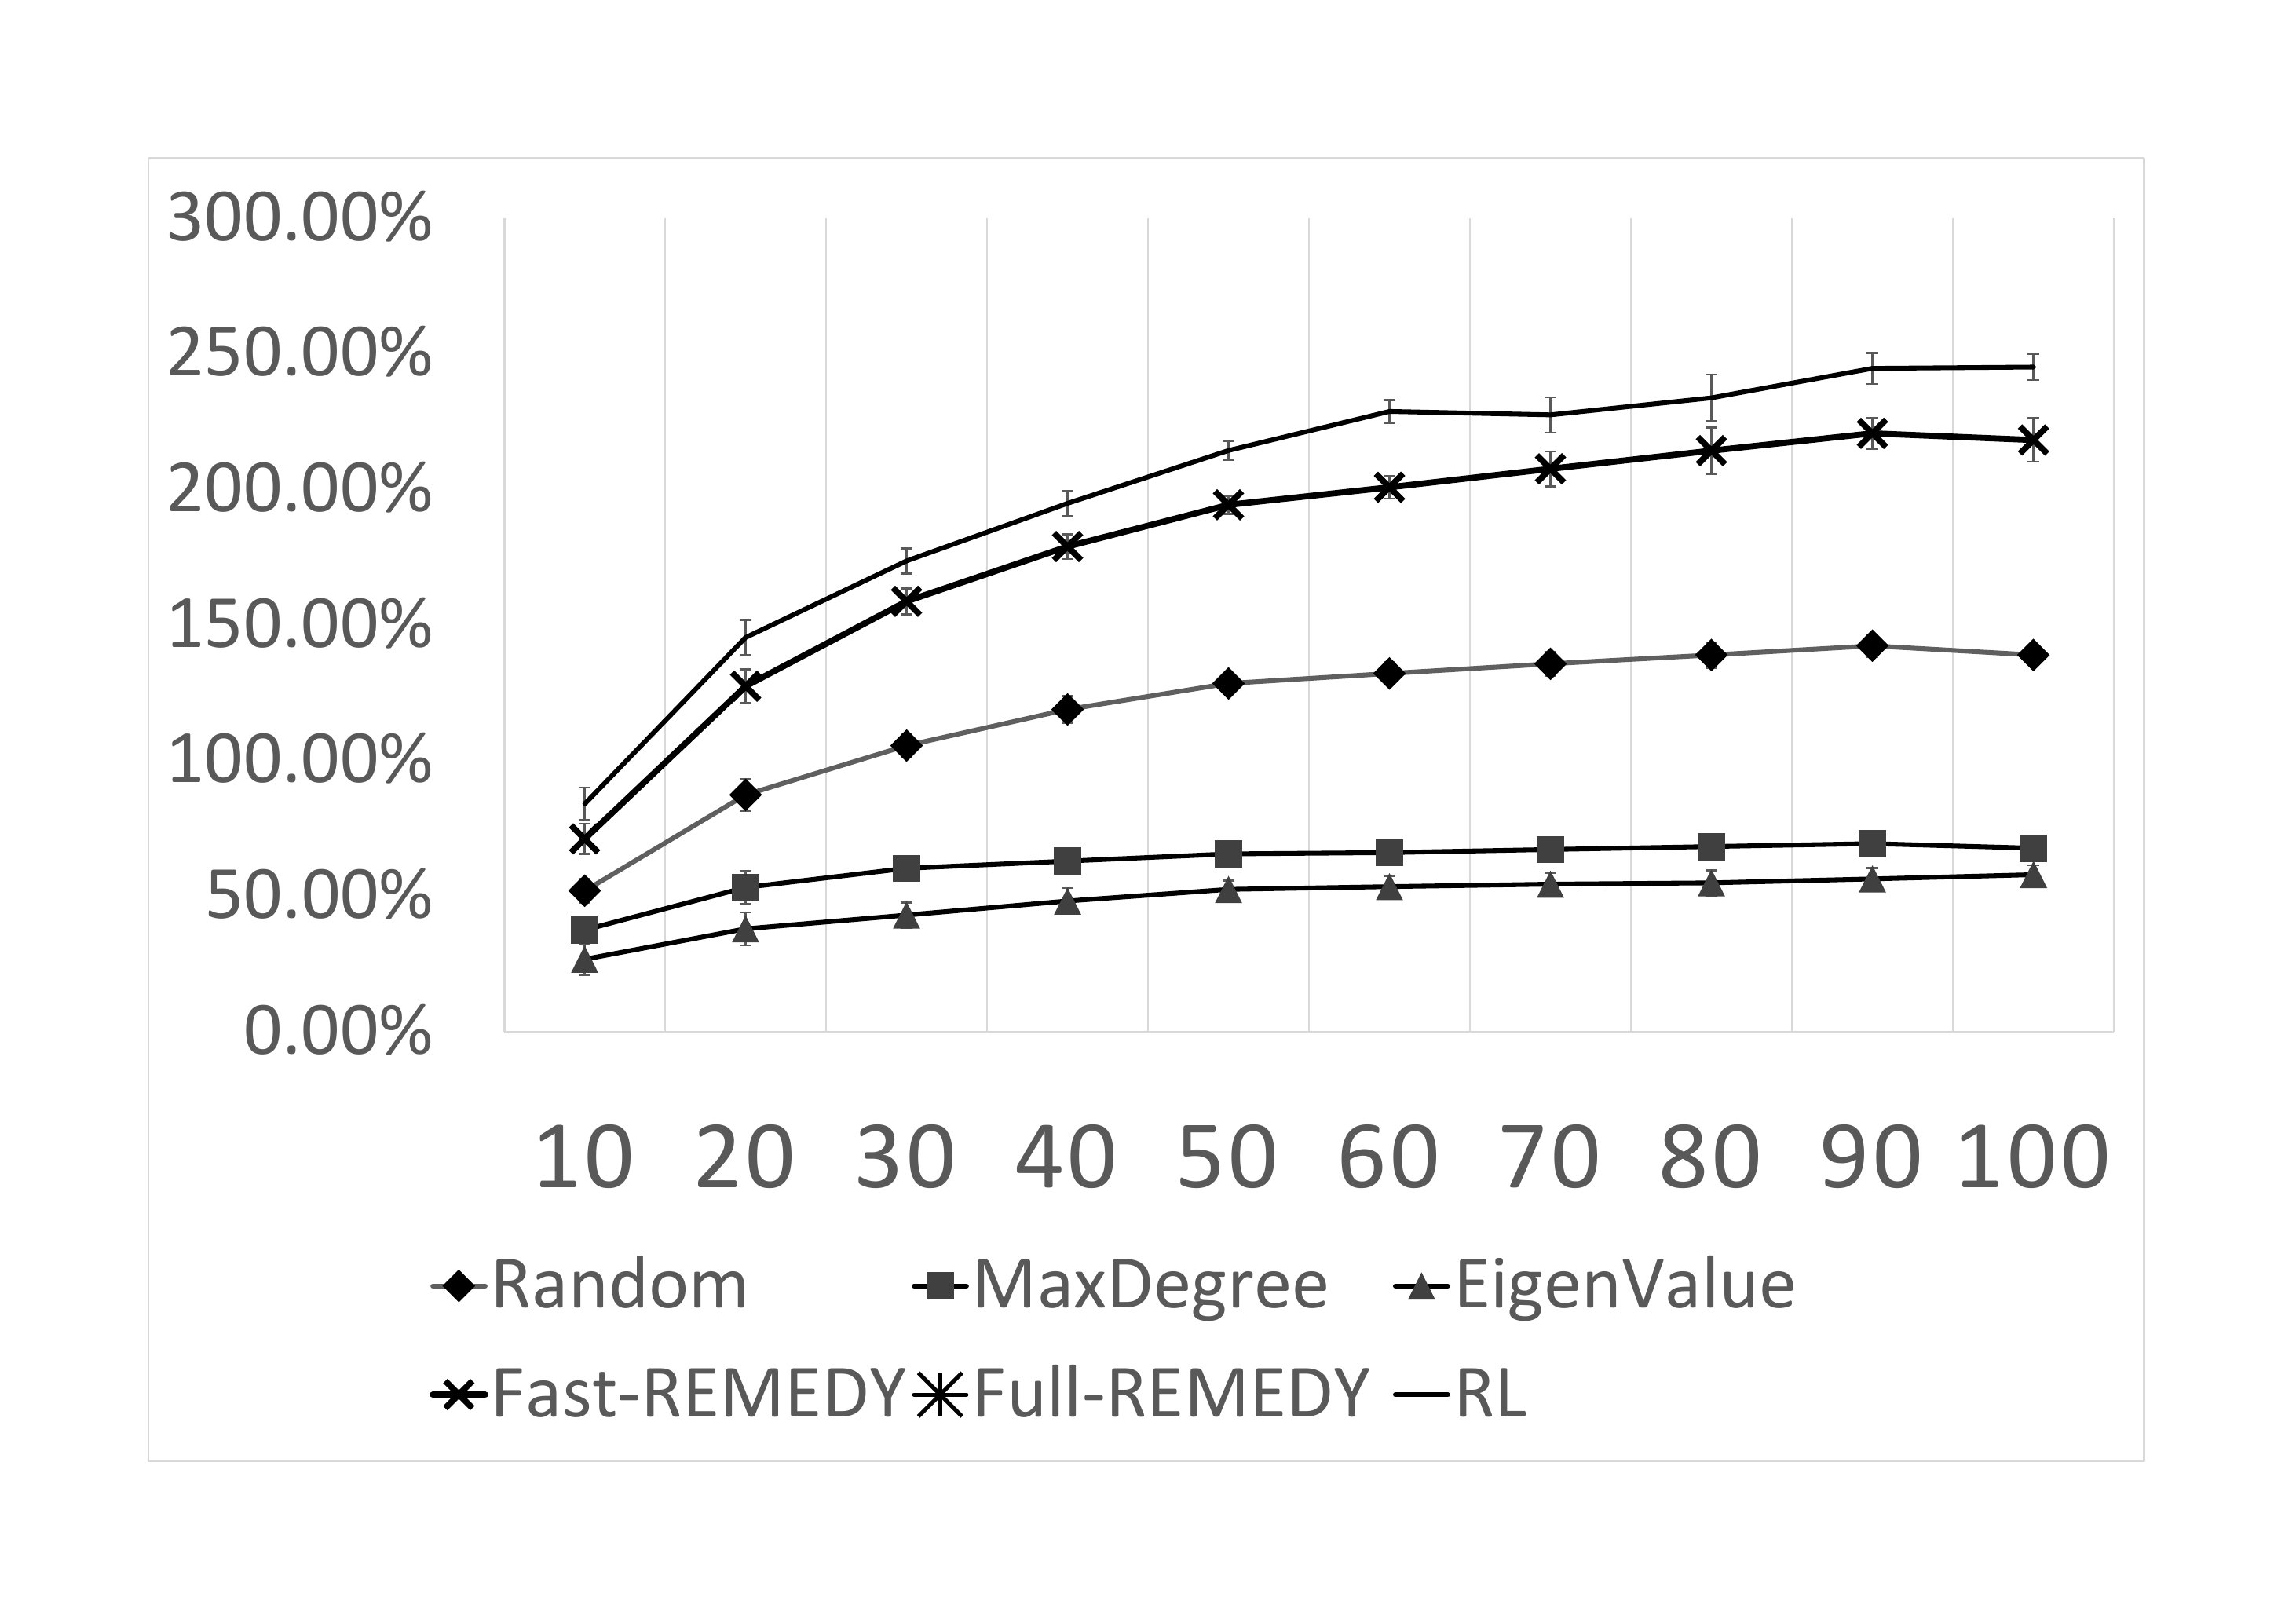}%
}\hfill
\subfloat[Flu]{%
  \includegraphics[width=0.35\textwidth,keepaspectratio]{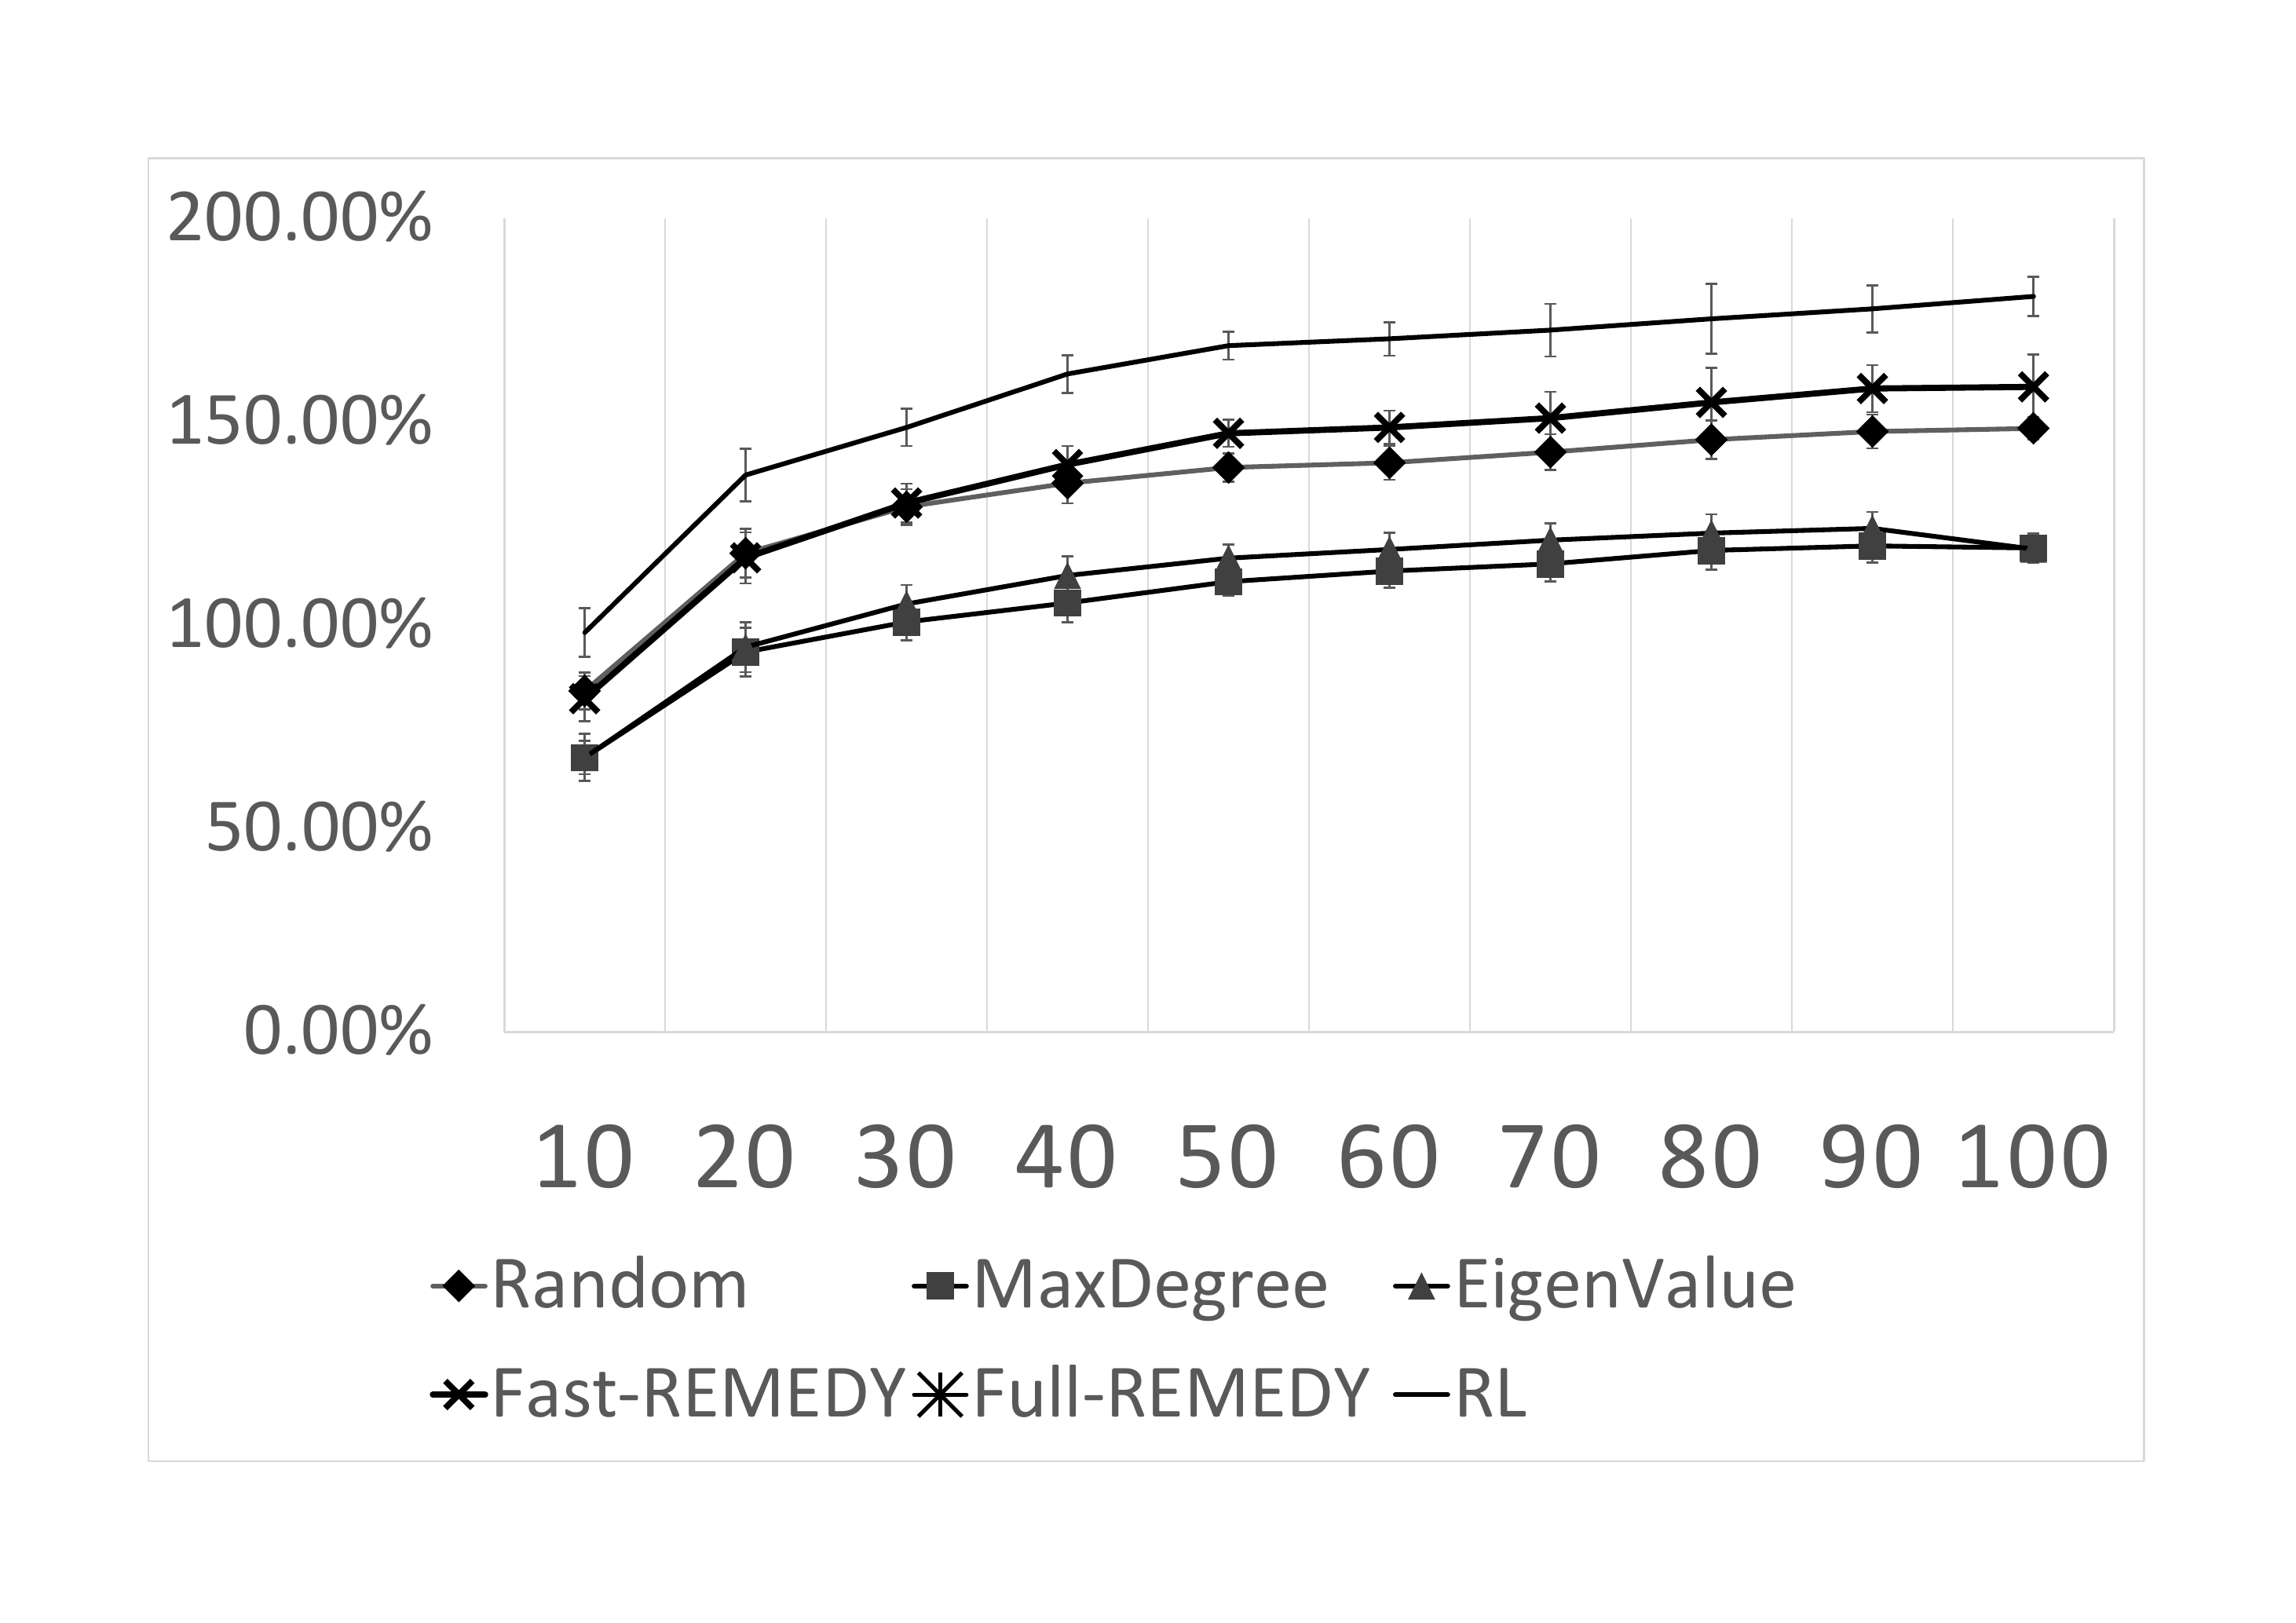}%
}\hfill
\subfloat[Irvine]{%
  \includegraphics[width=0.35\textwidth,keepaspectratio]{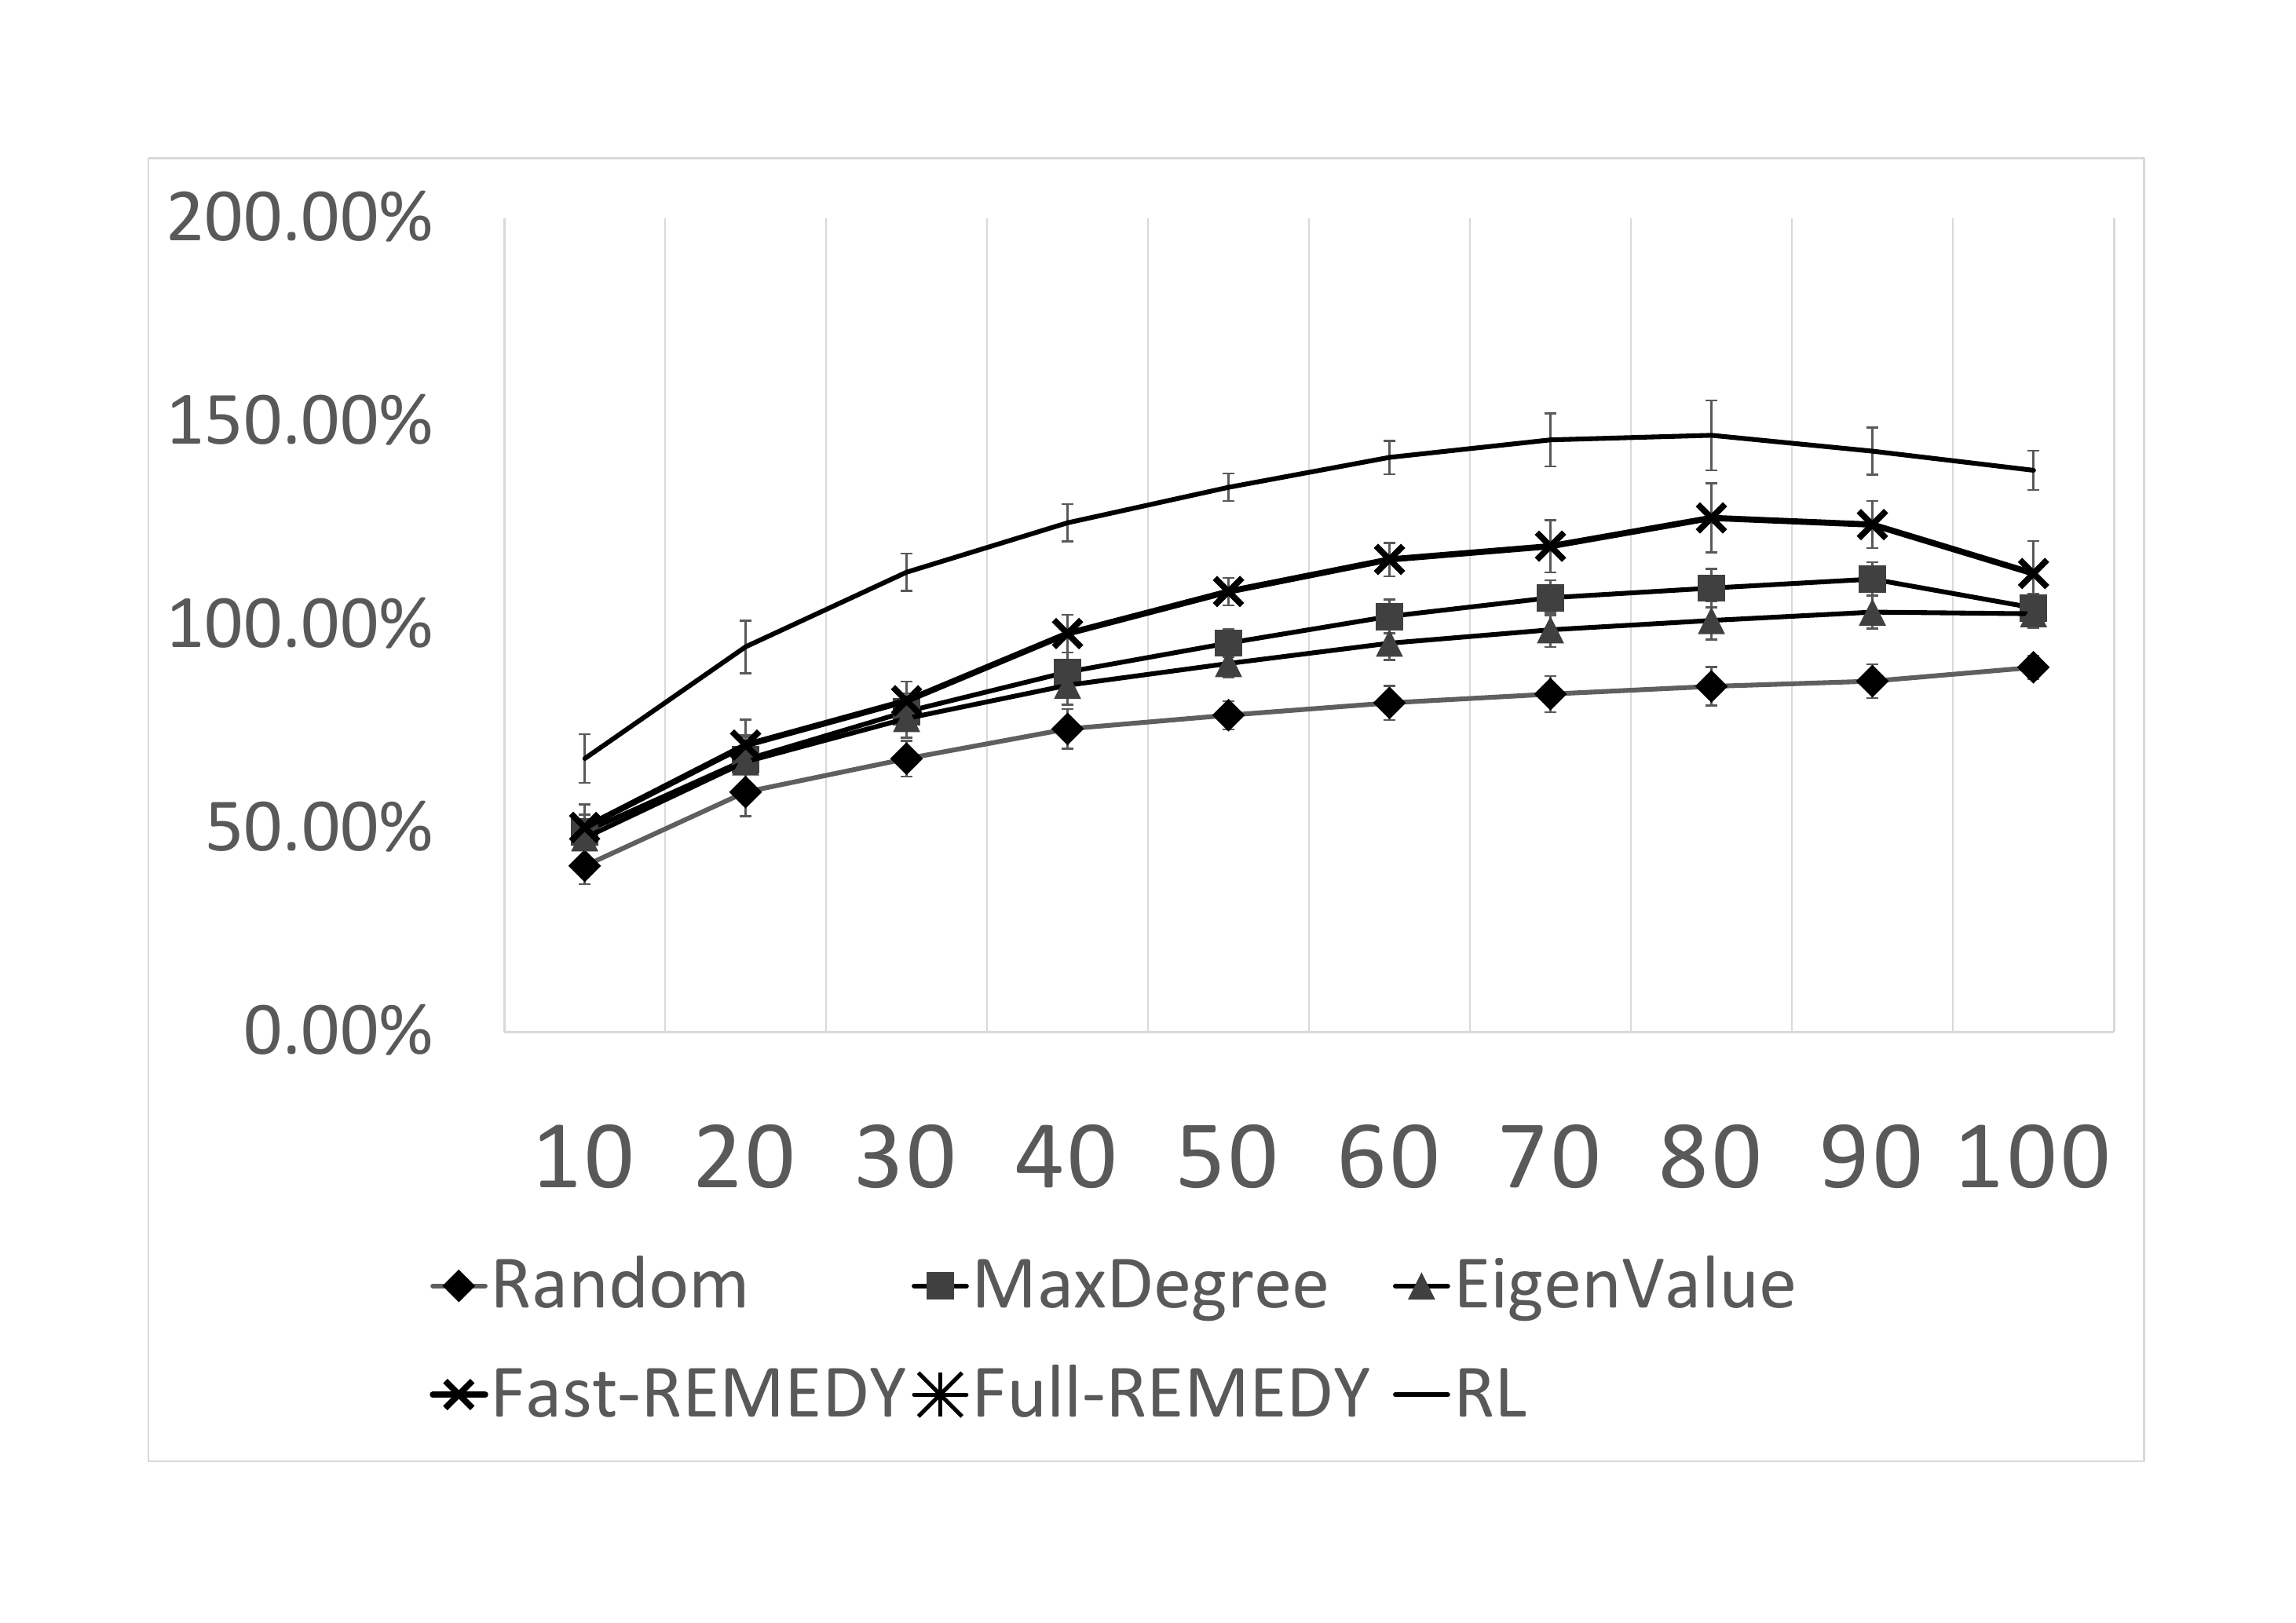}%
}\hfill
\centering
\caption{Performance under node information removal.}\label{timev}
\end{figure*}

\begin{figure*}[t]
\centering
\subfloat[Hospital]{%
  \includegraphics[width=0.35\textwidth,keepaspectratio]{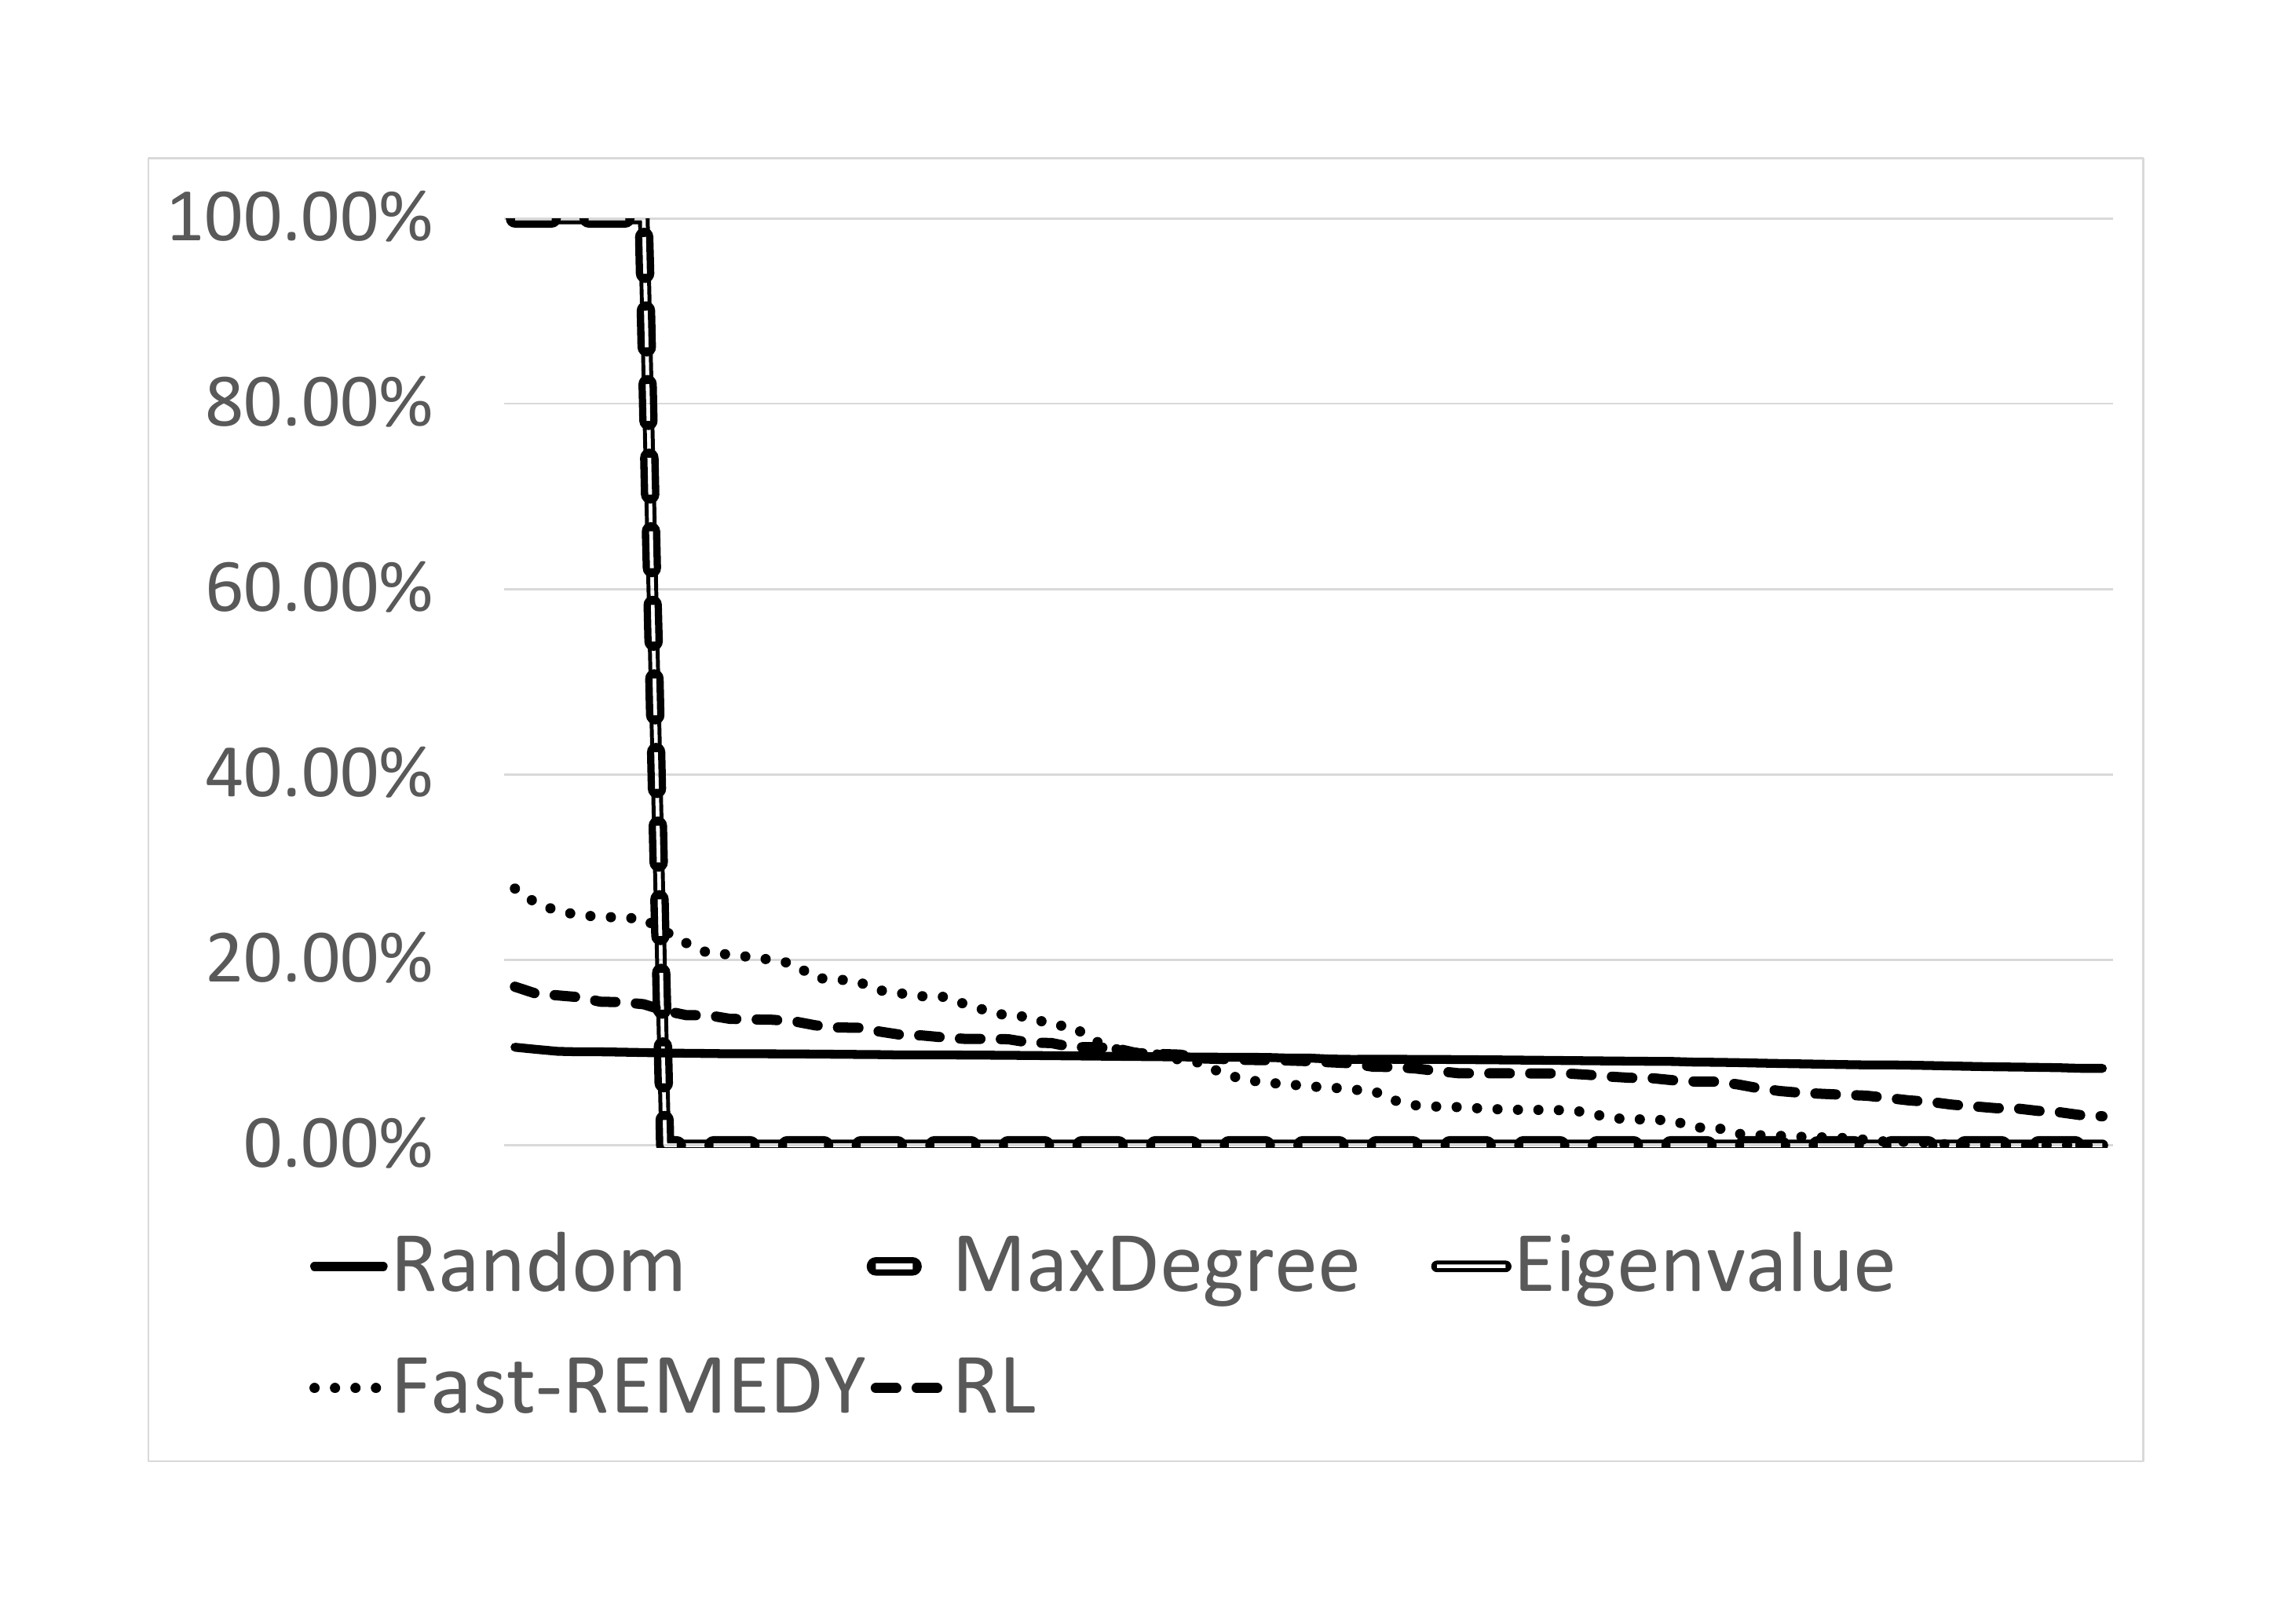}%
}\hfill
\subfloat[India]{%
  \includegraphics[width=0.35\textwidth,keepaspectratio]{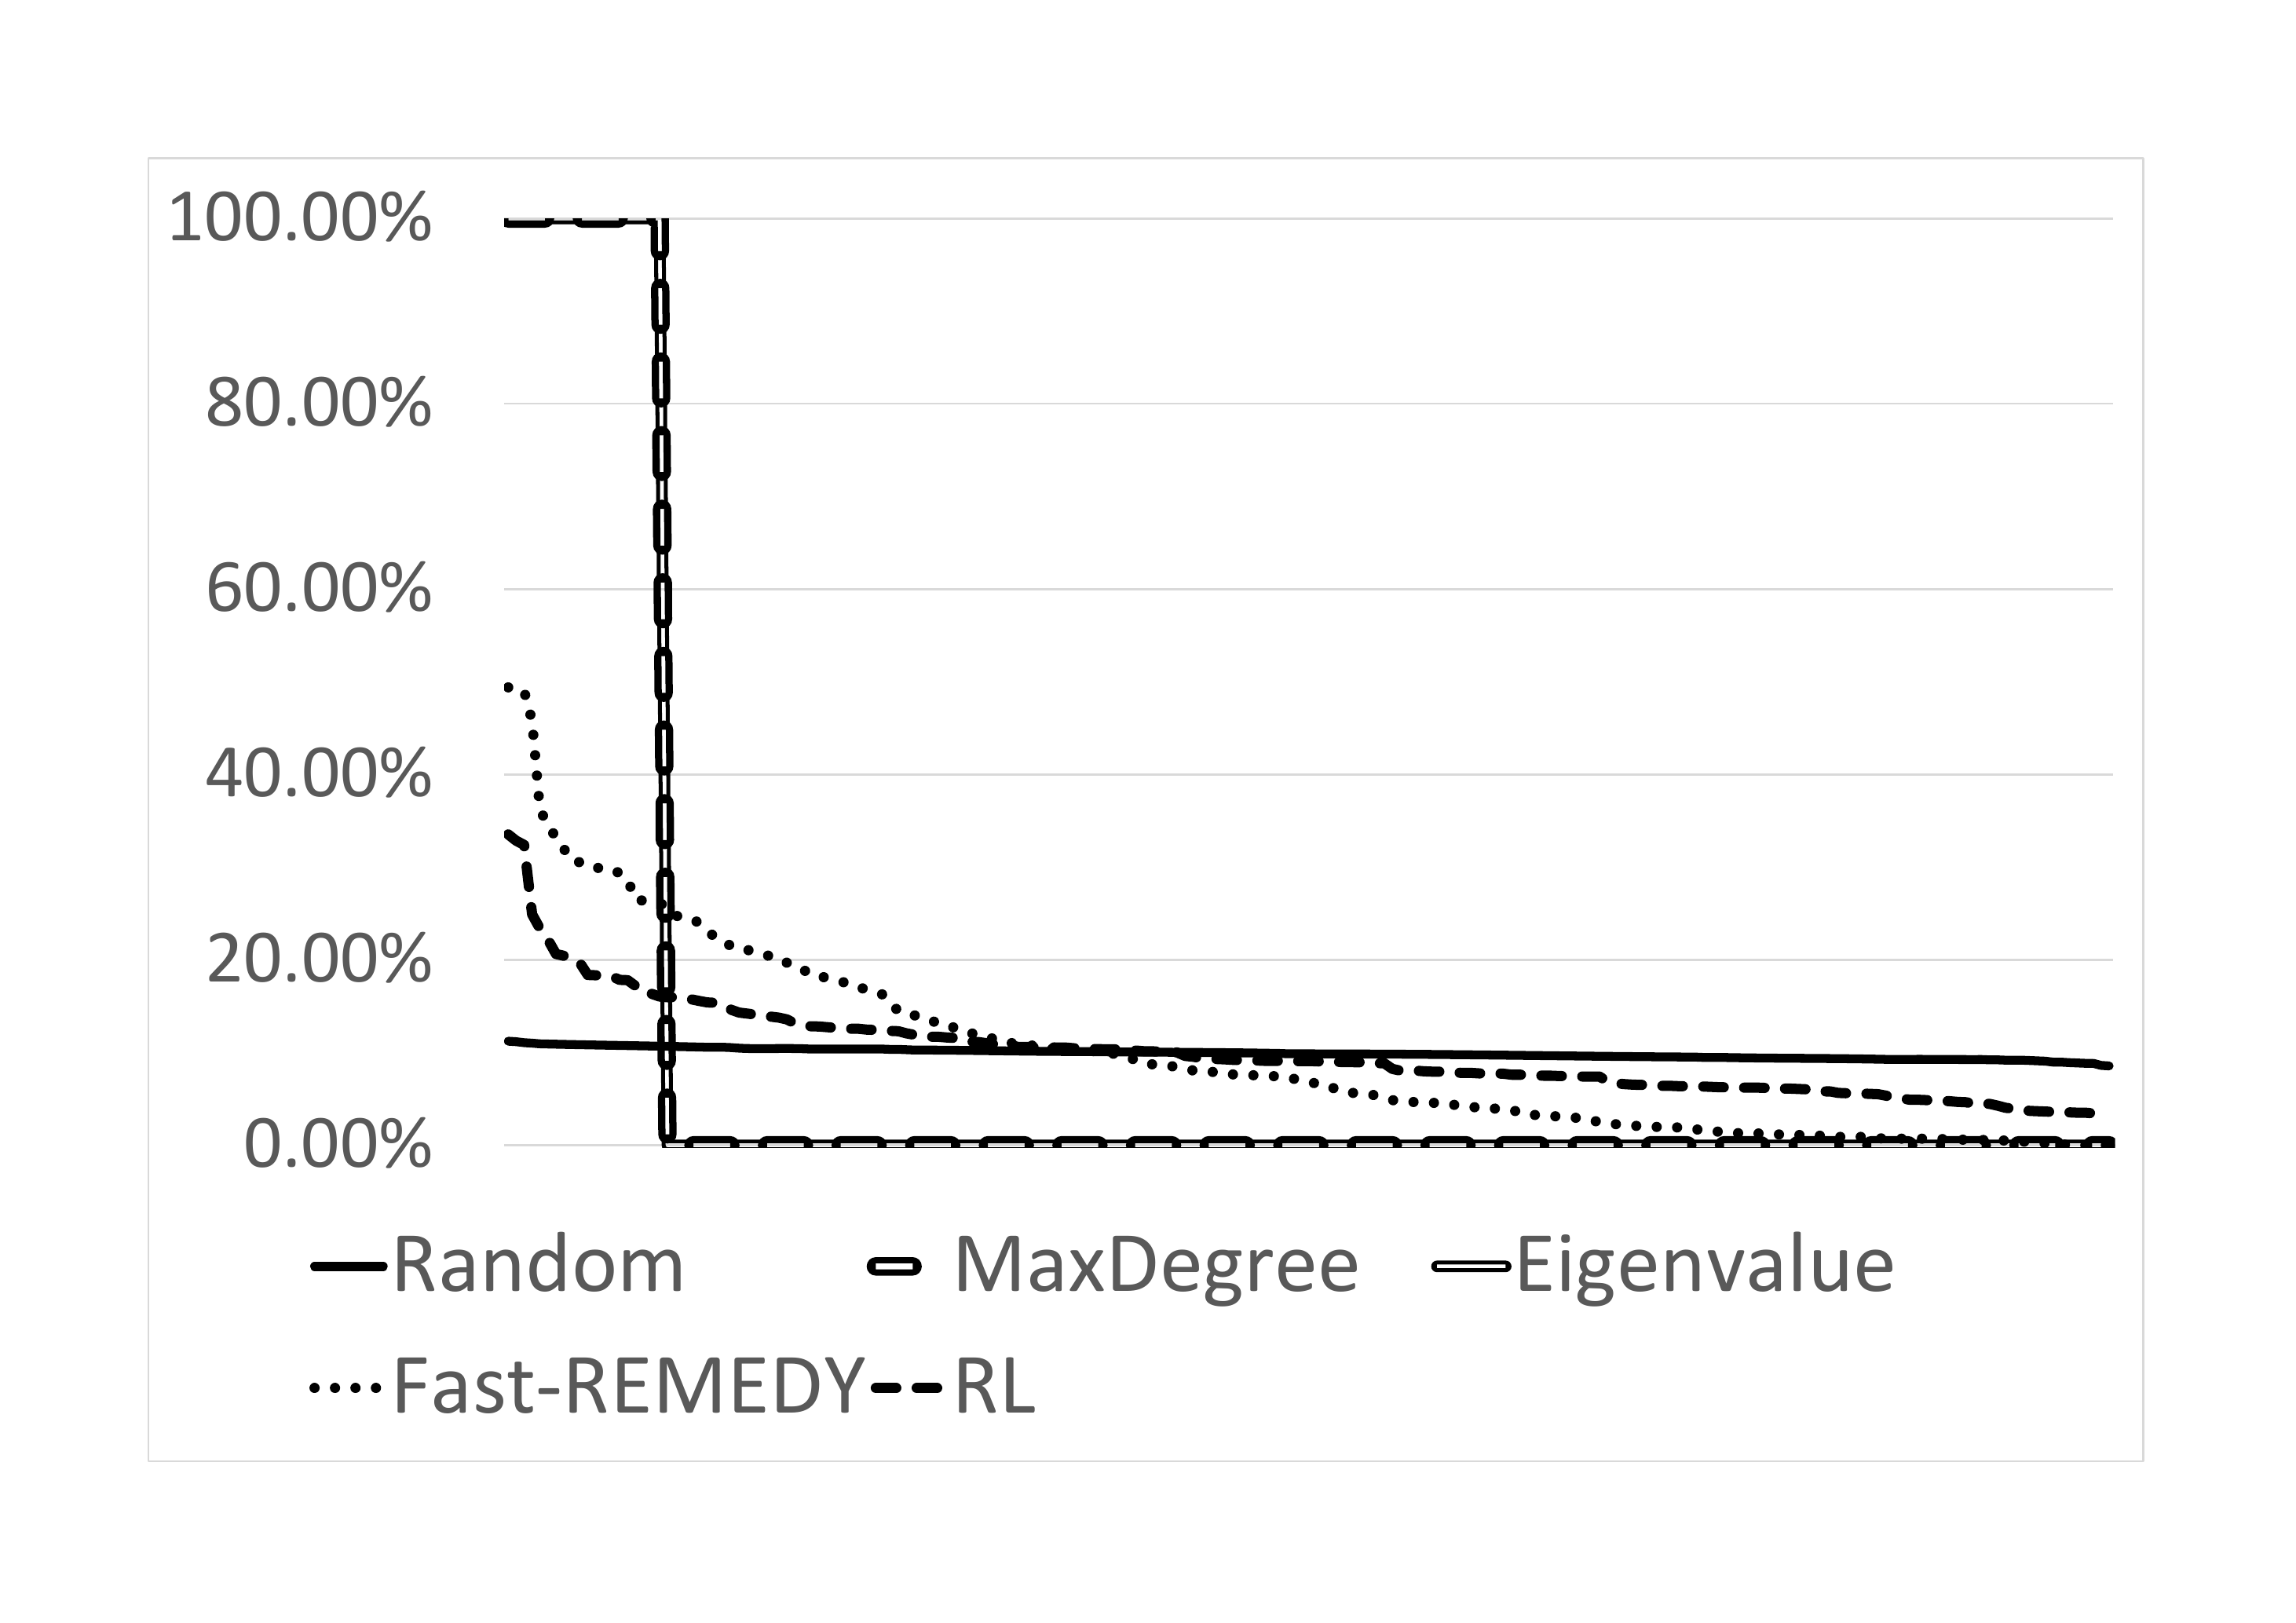}%
}\hfill
\subfloat[Flu]{%
  \includegraphics[width=0.35\textwidth,keepaspectratio]{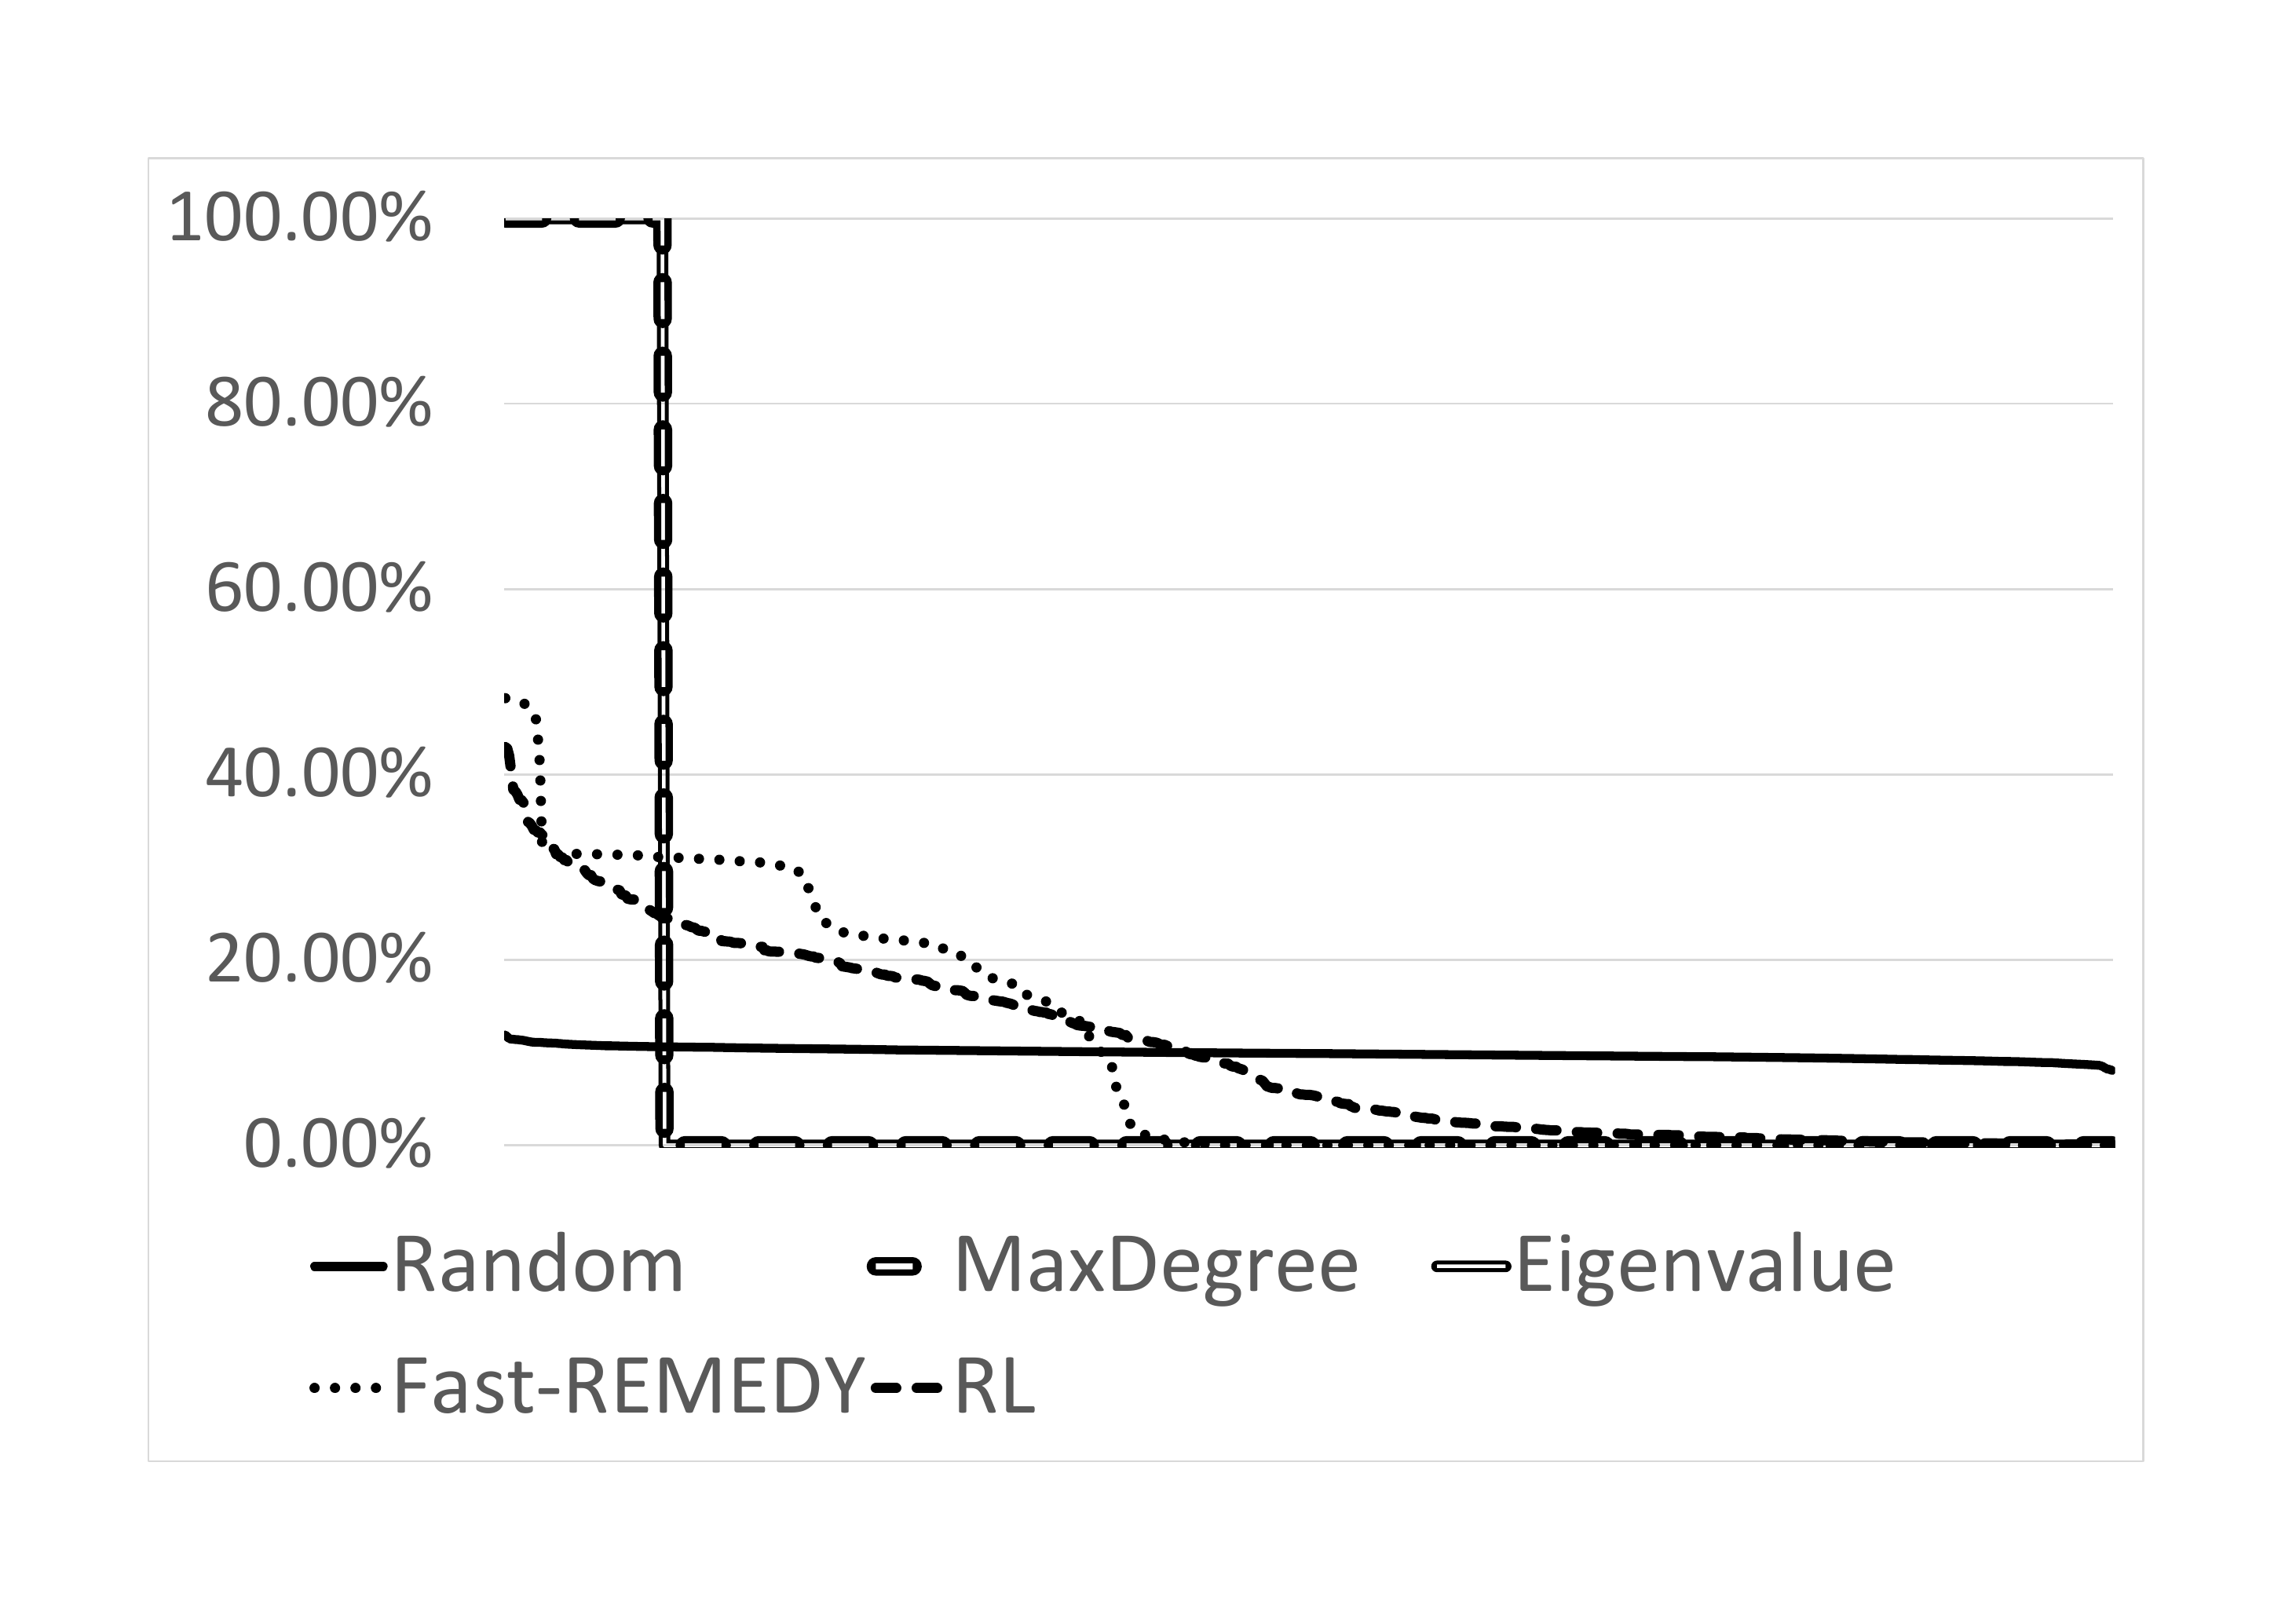}%
}\hfill
\subfloat[Flu]{%
  \includegraphics[width=0.35\textwidth,keepaspectratio]{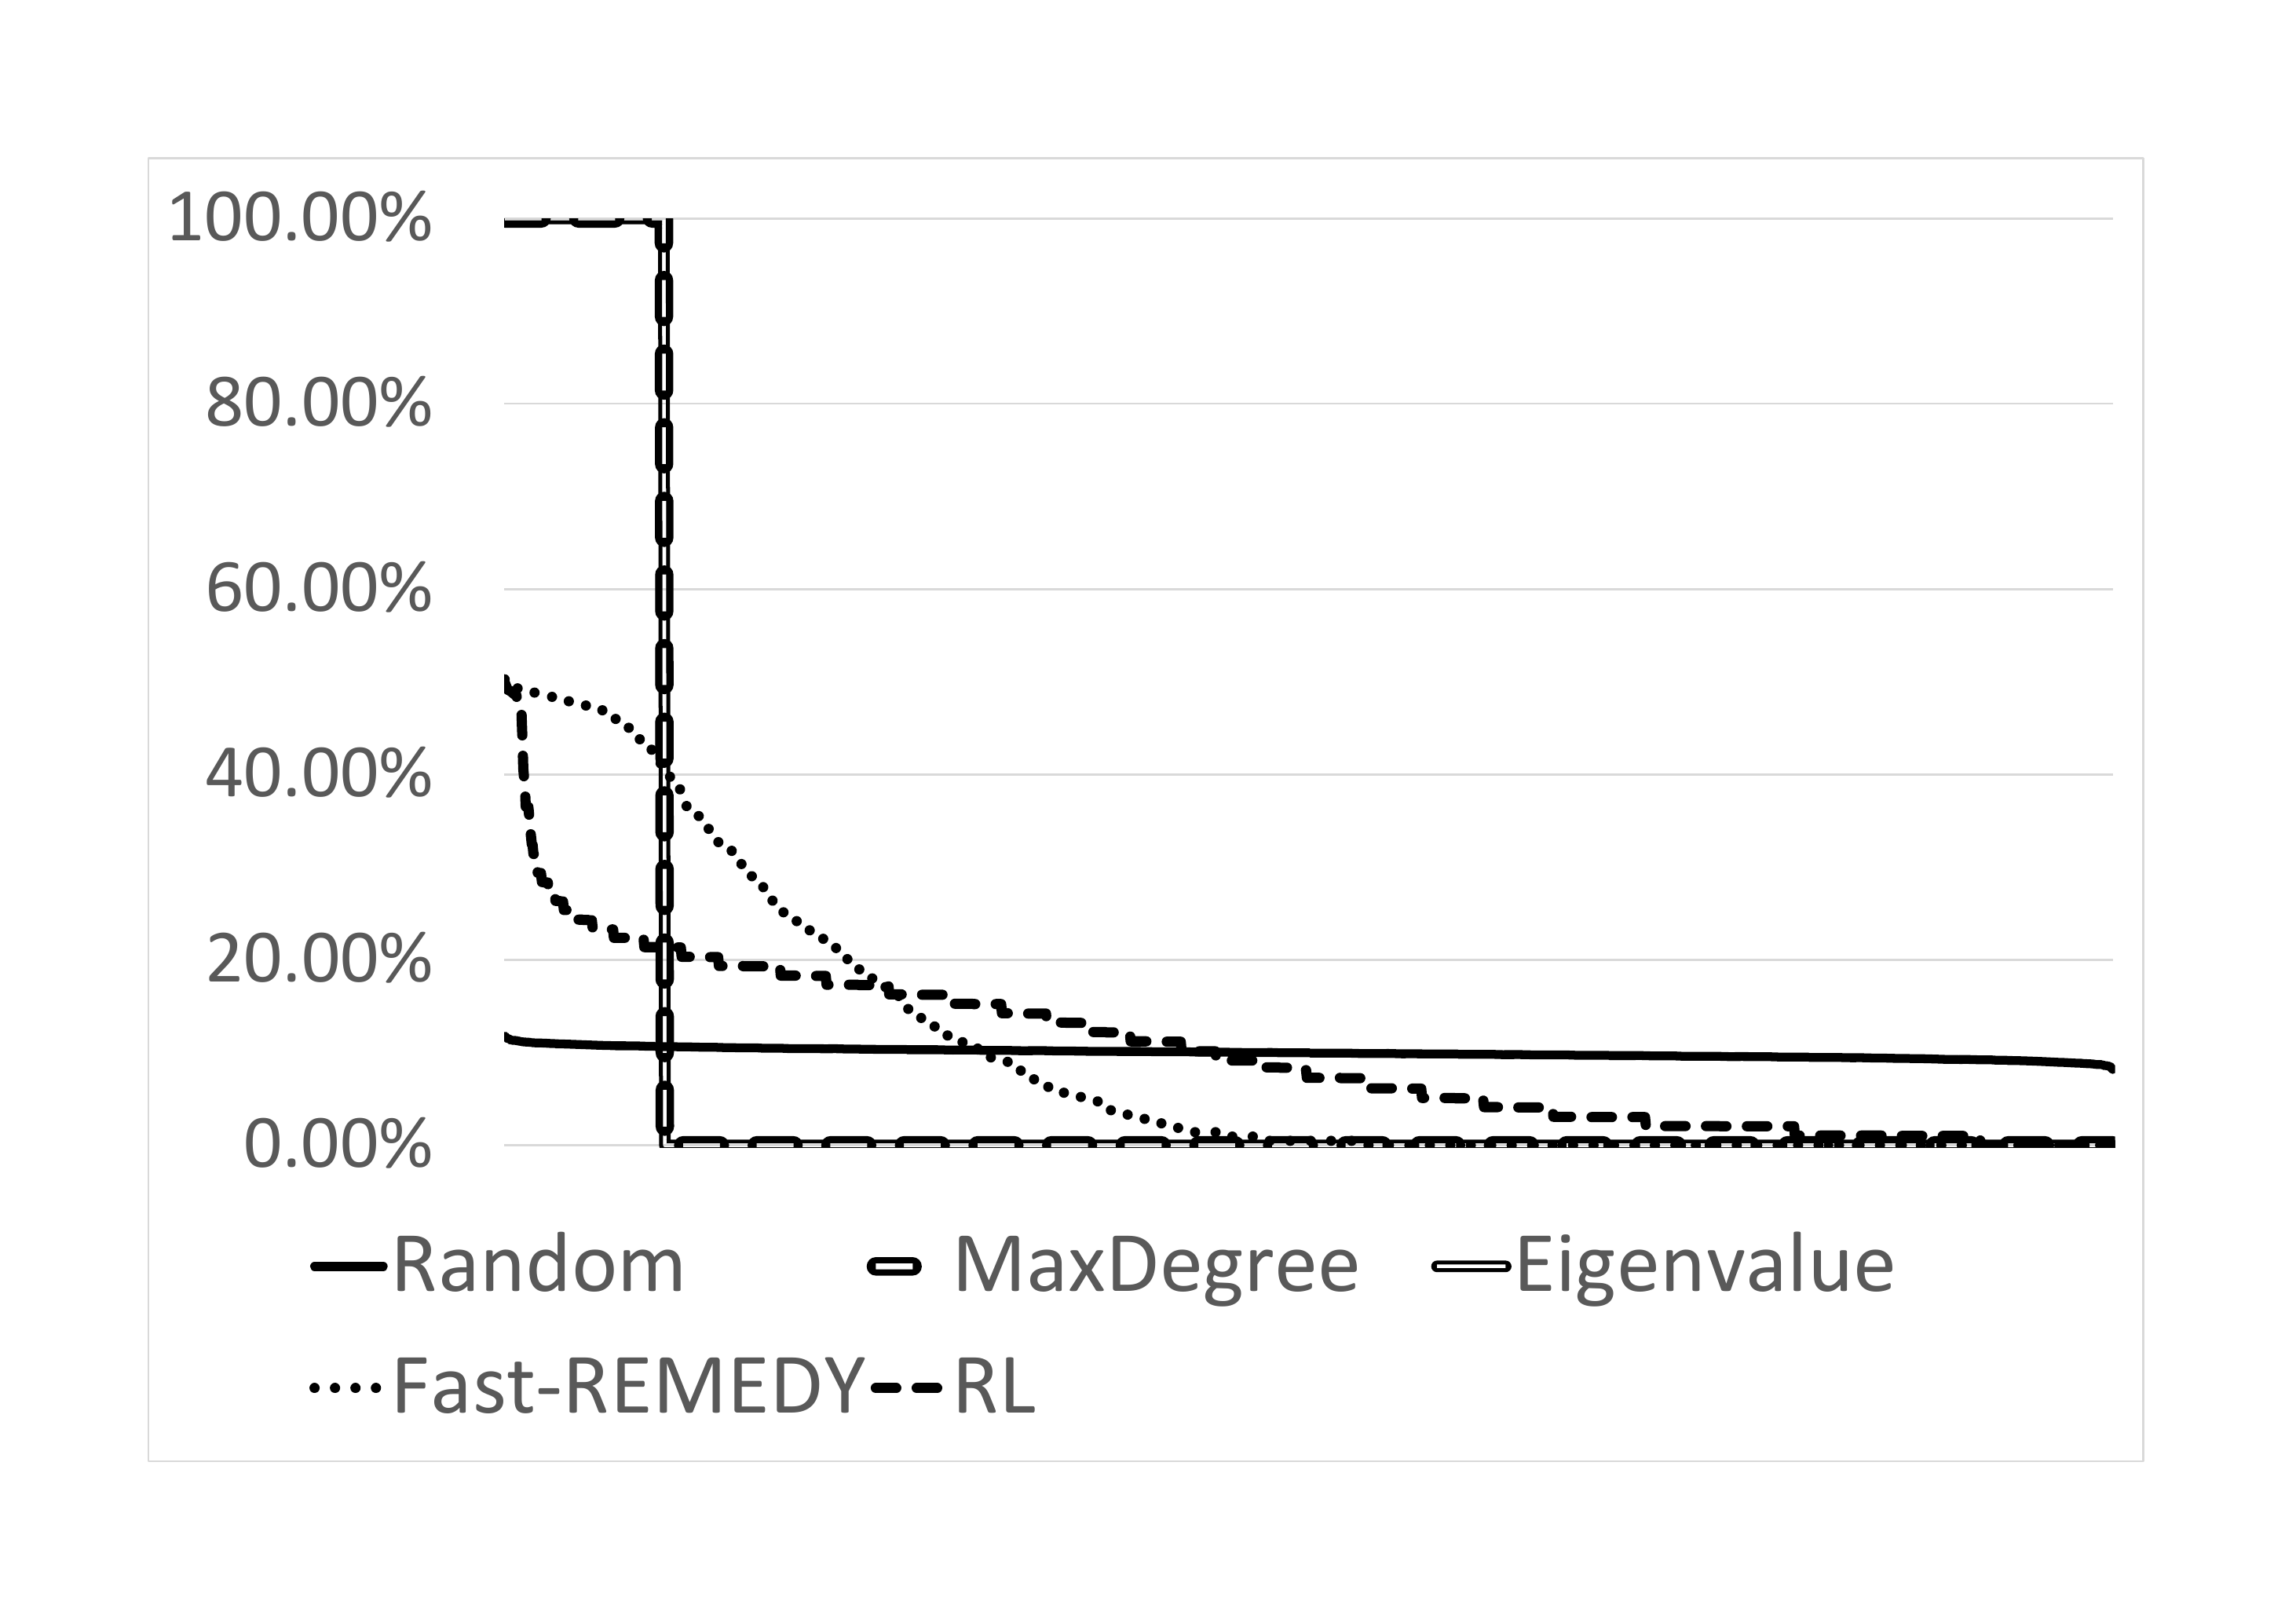}%
}\hfill
\centering
\caption{Node picking frequency.}\label{freq}
\end{figure*}

\begin{figure*}[t]
\centering
\subfloat[Hospital]{%
  \includegraphics[width=0.35\textwidth,keepaspectratio]{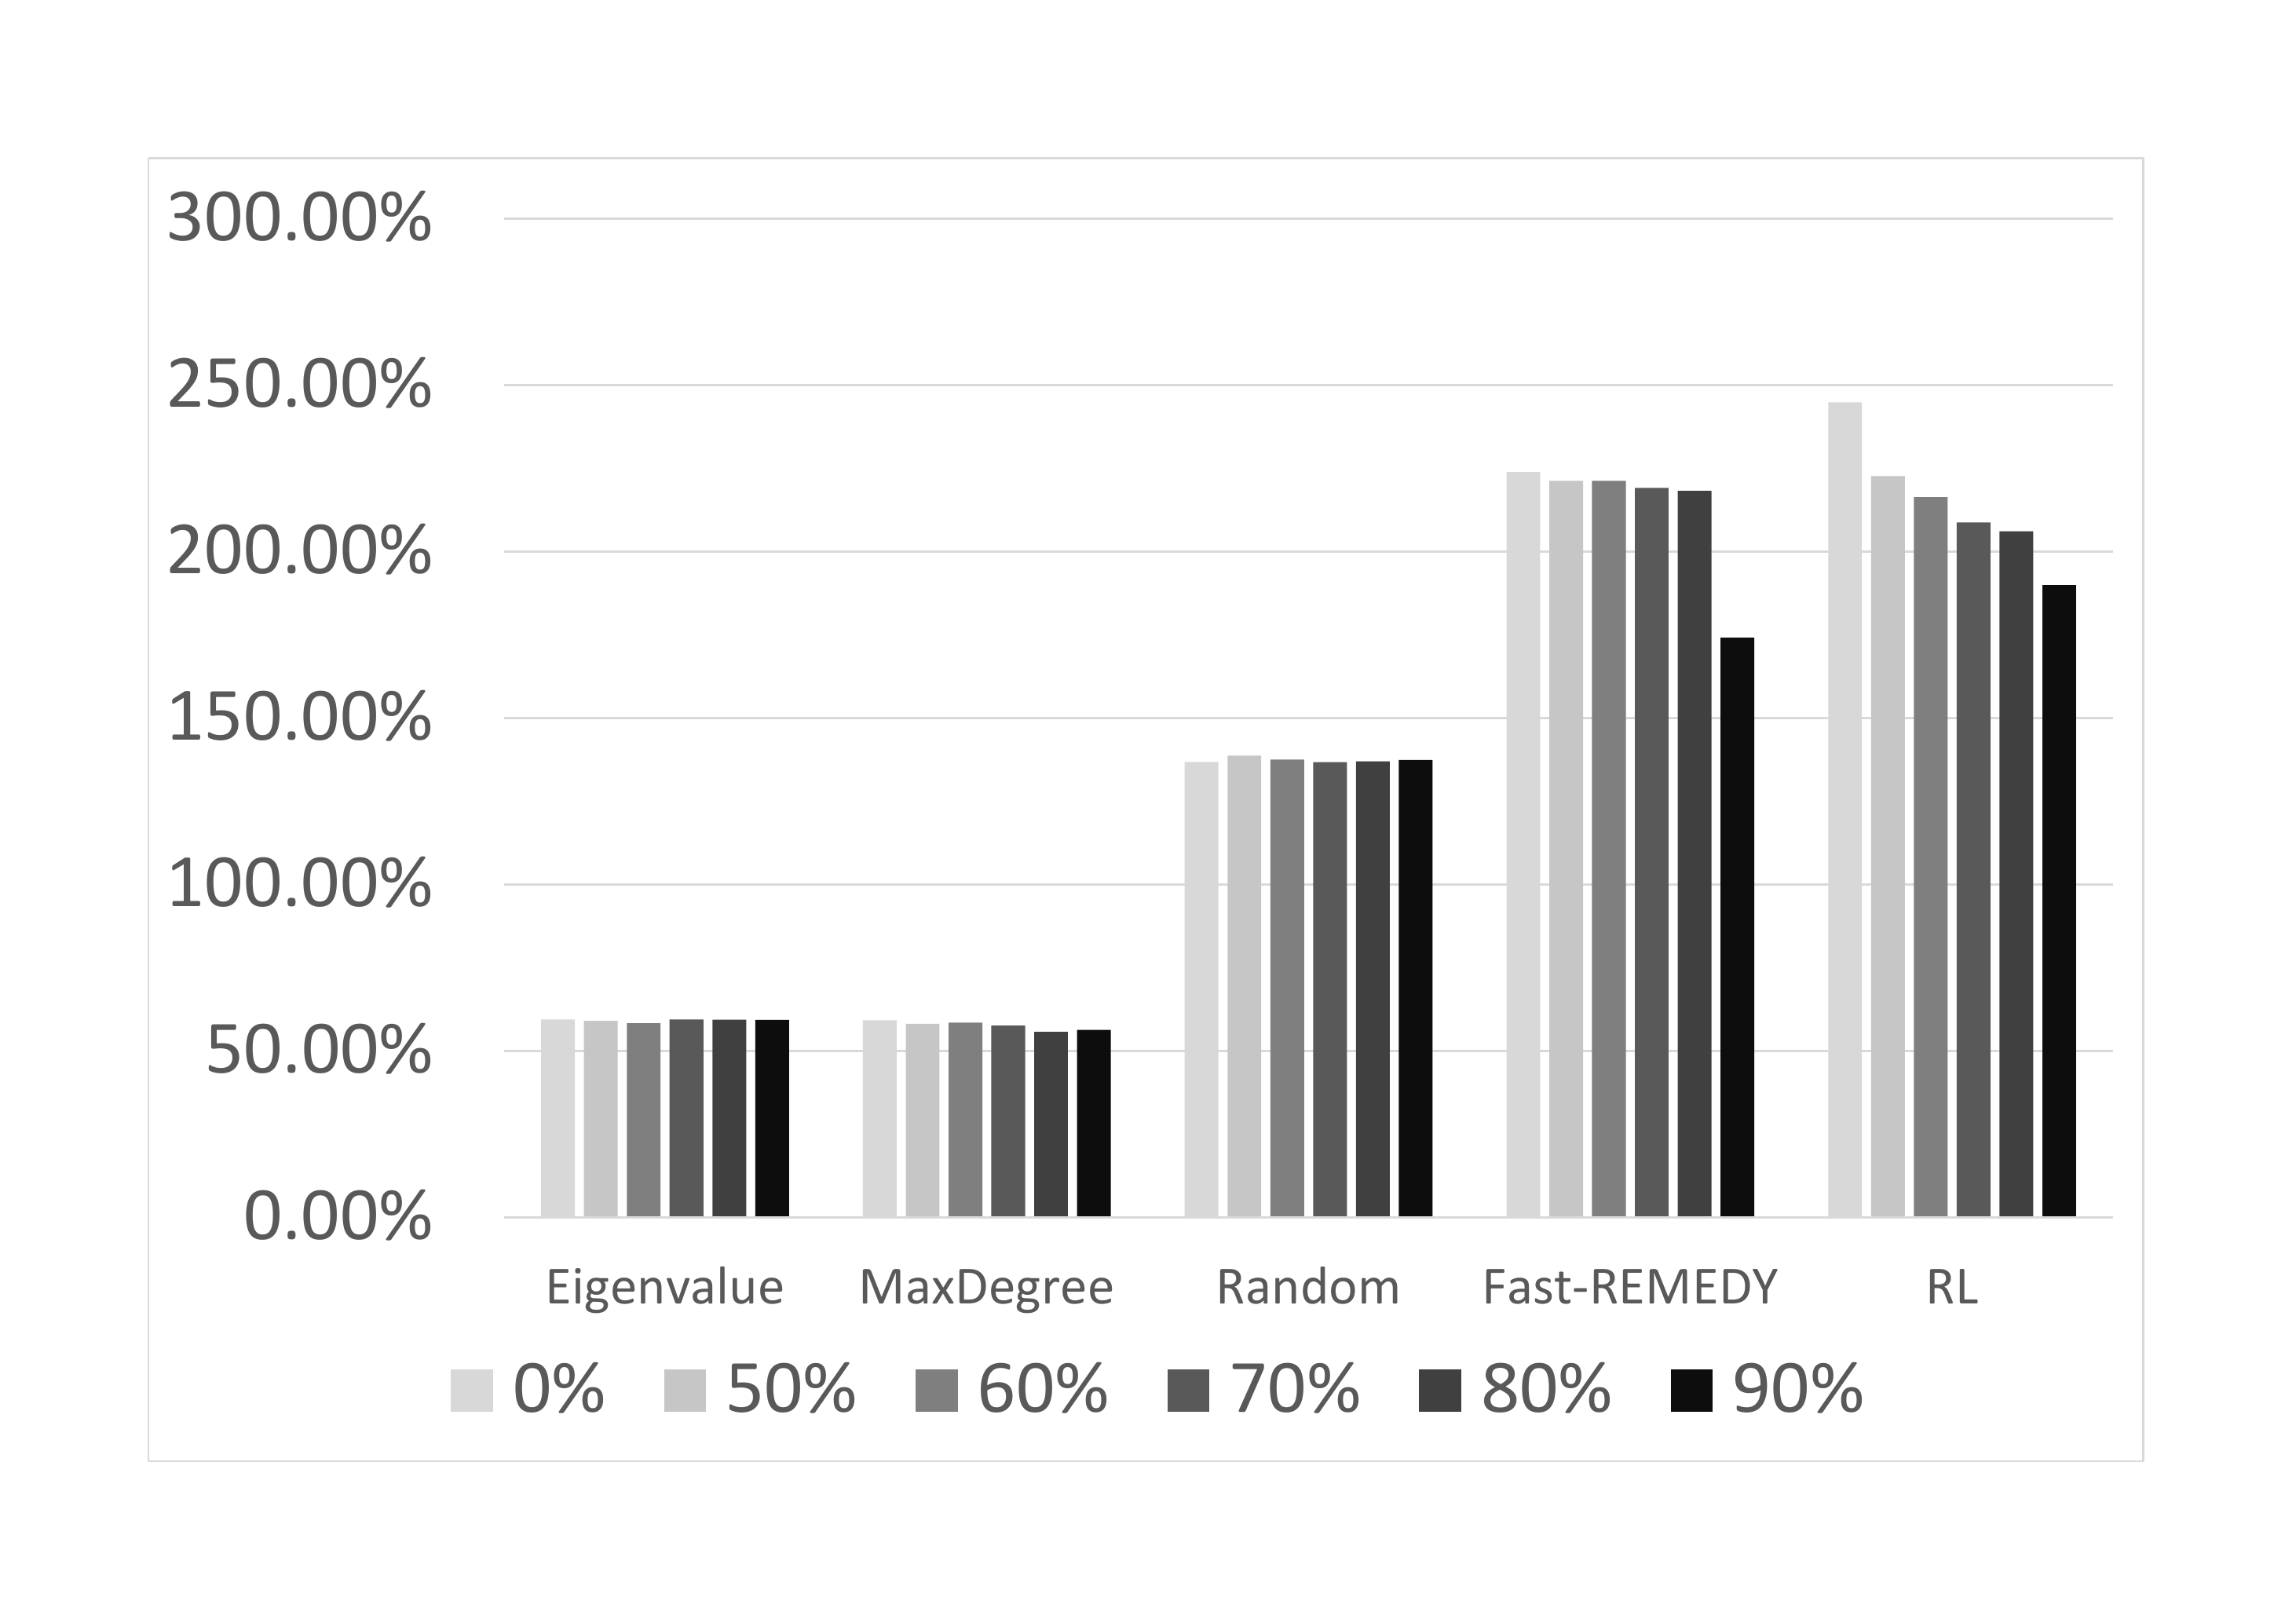}%
}\hfill
\subfloat[India]{%
  \includegraphics[width=0.35\textwidth,keepaspectratio]{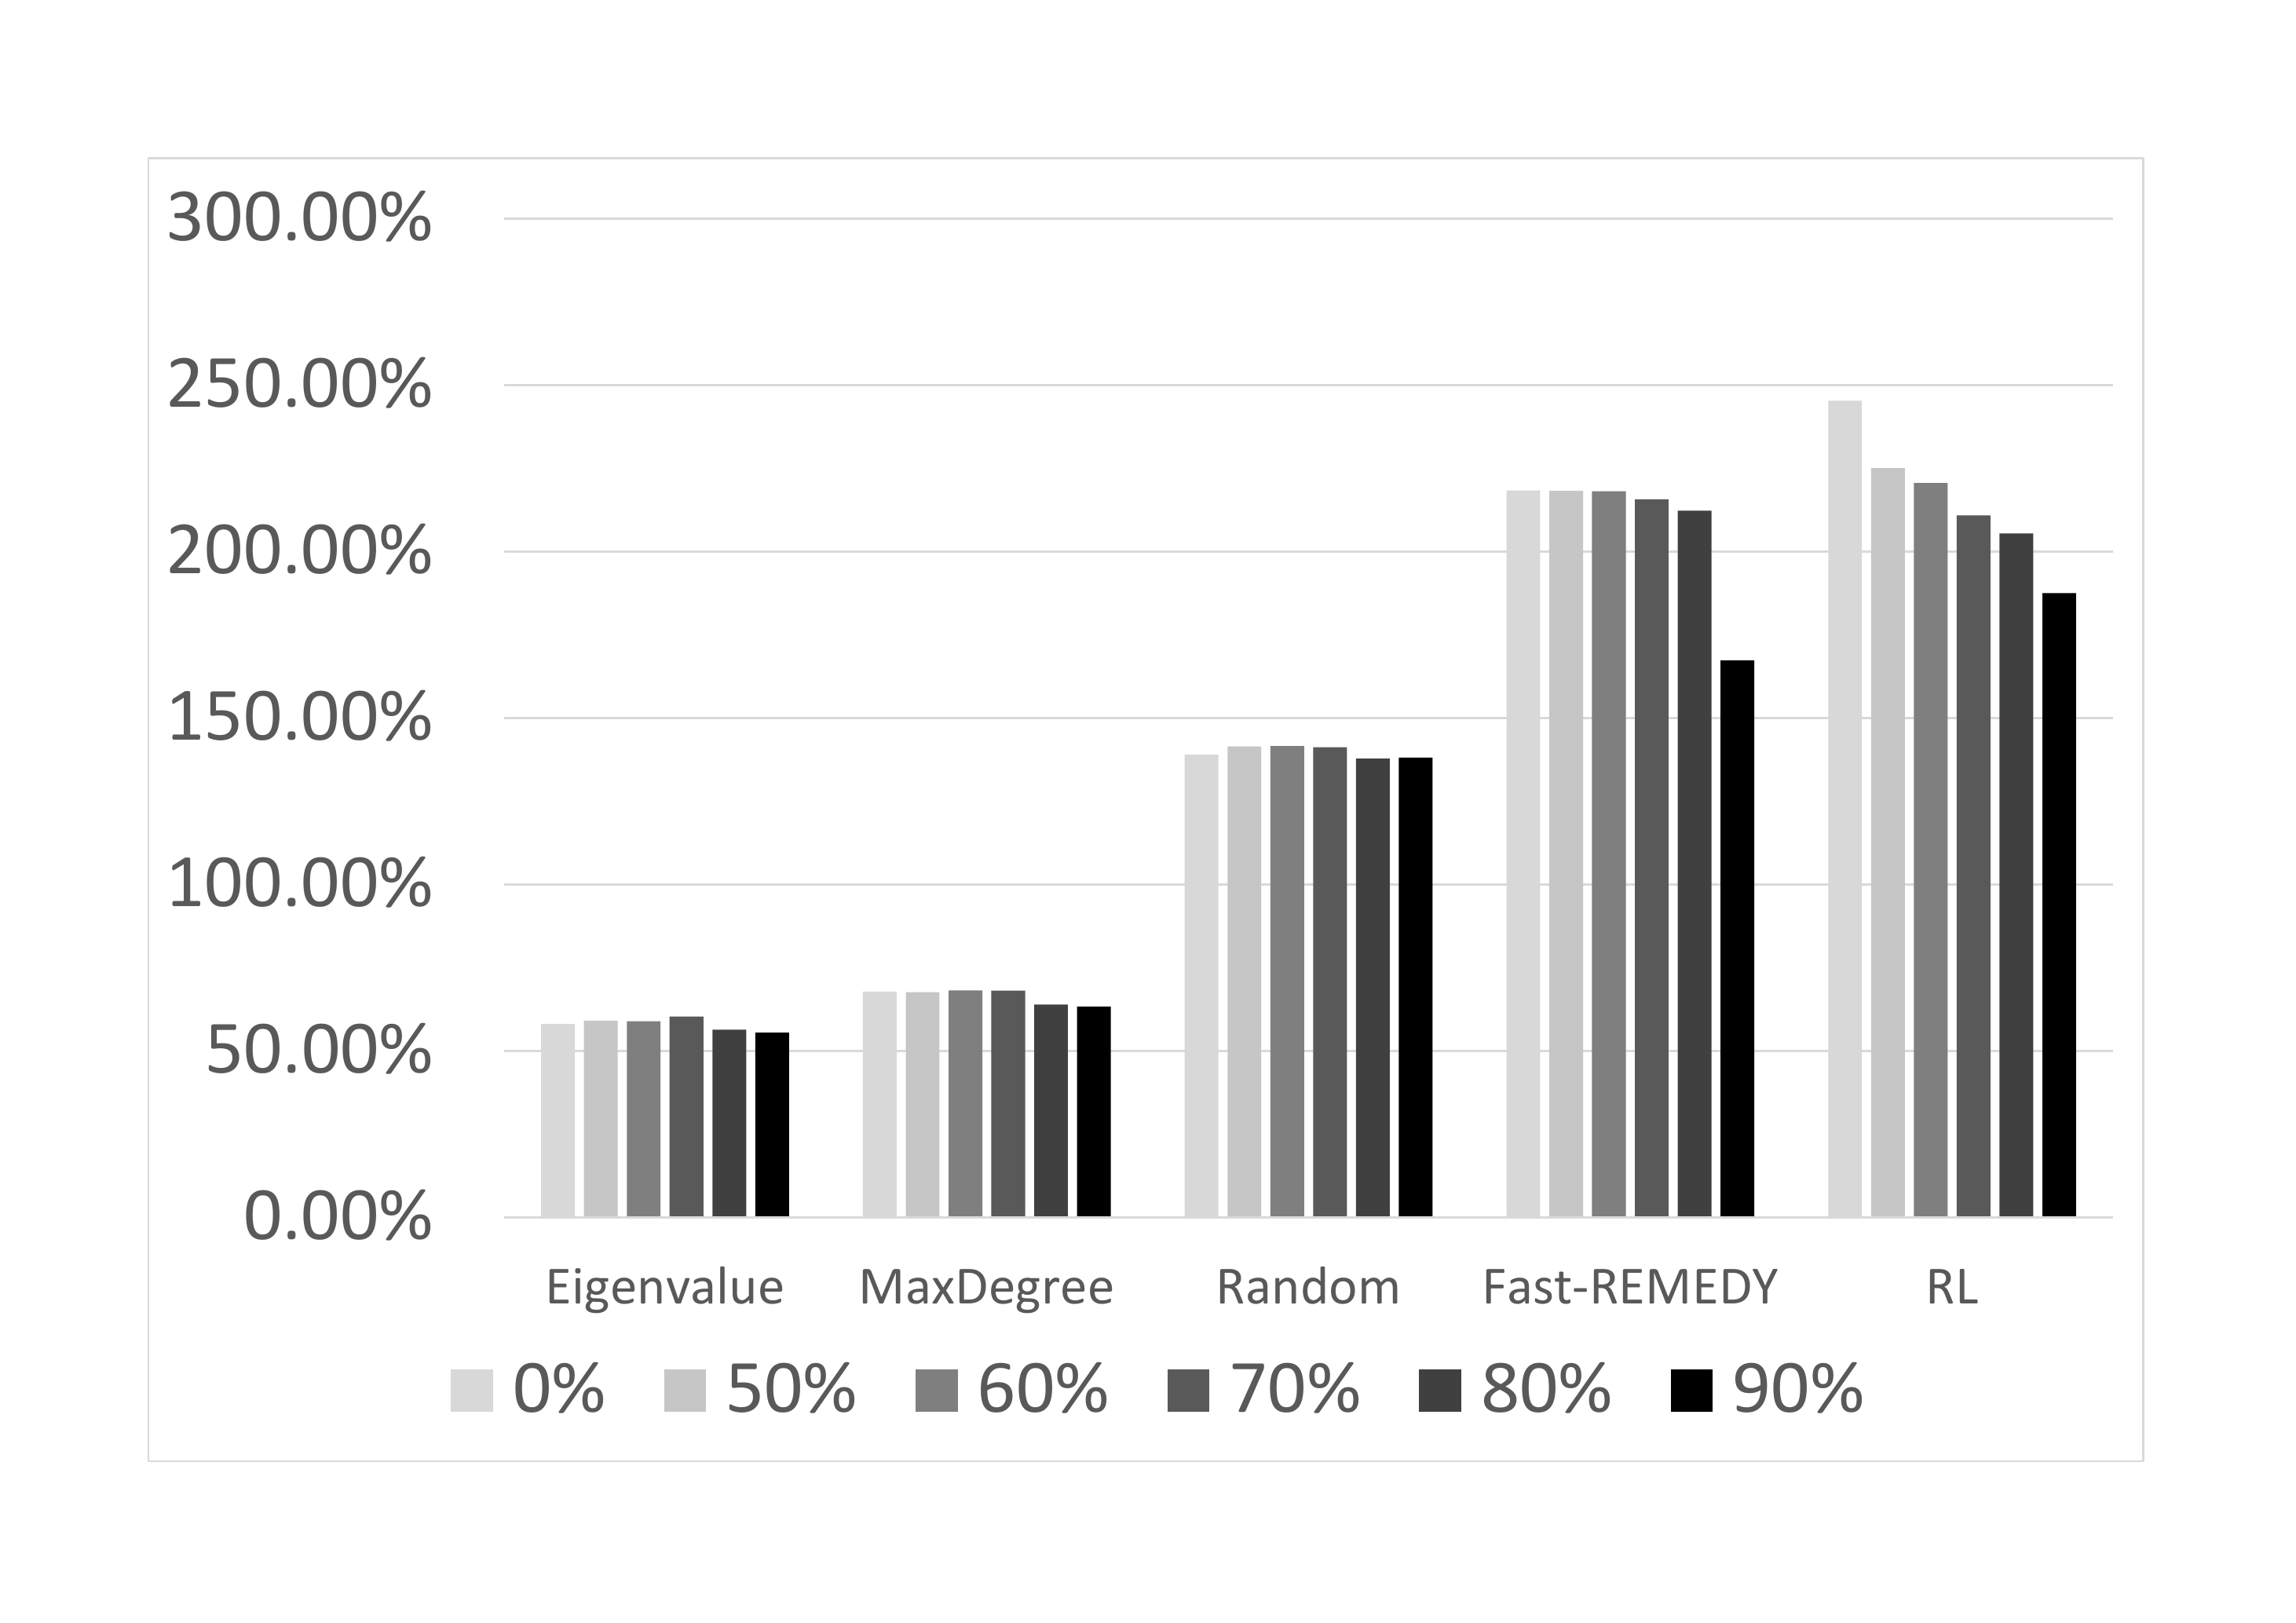}%
}\hfill
\subfloat[Flu]{%
  \includegraphics[width=0.35\textwidth,keepaspectratio]{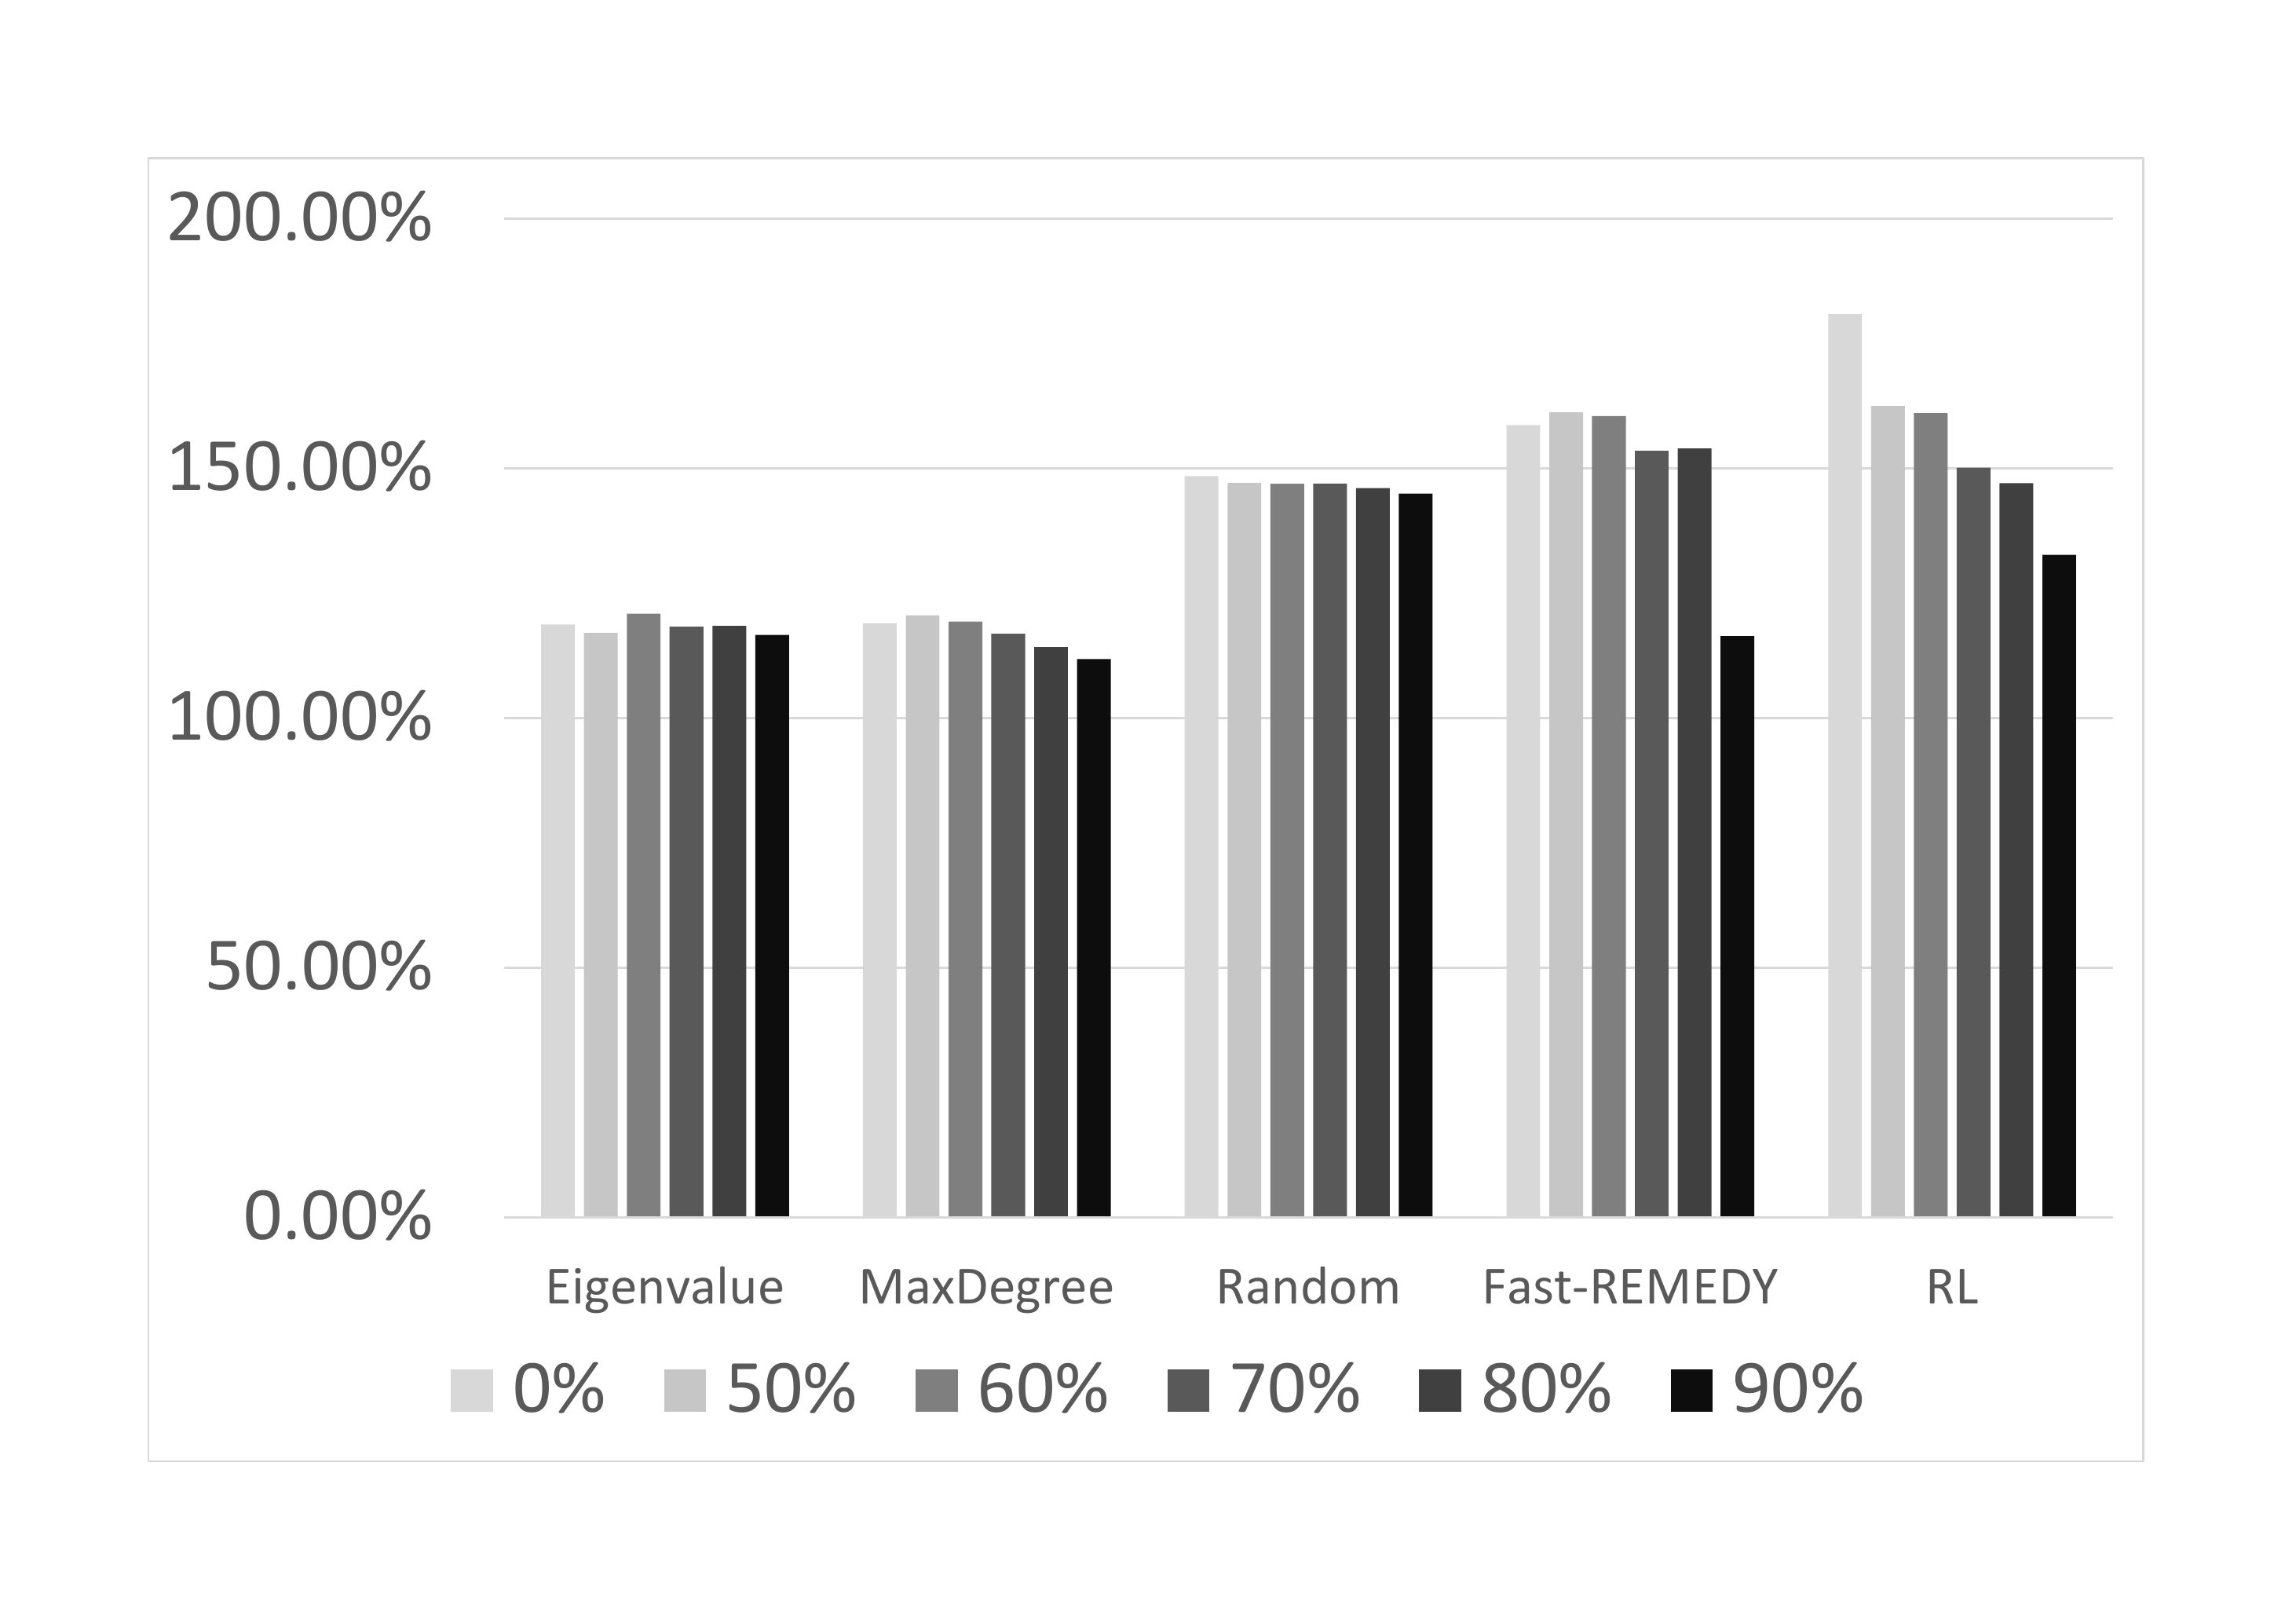}%
}\hfill
\subfloat[Irvine]{%
  \includegraphics[width=0.35\textwidth,keepaspectratio]{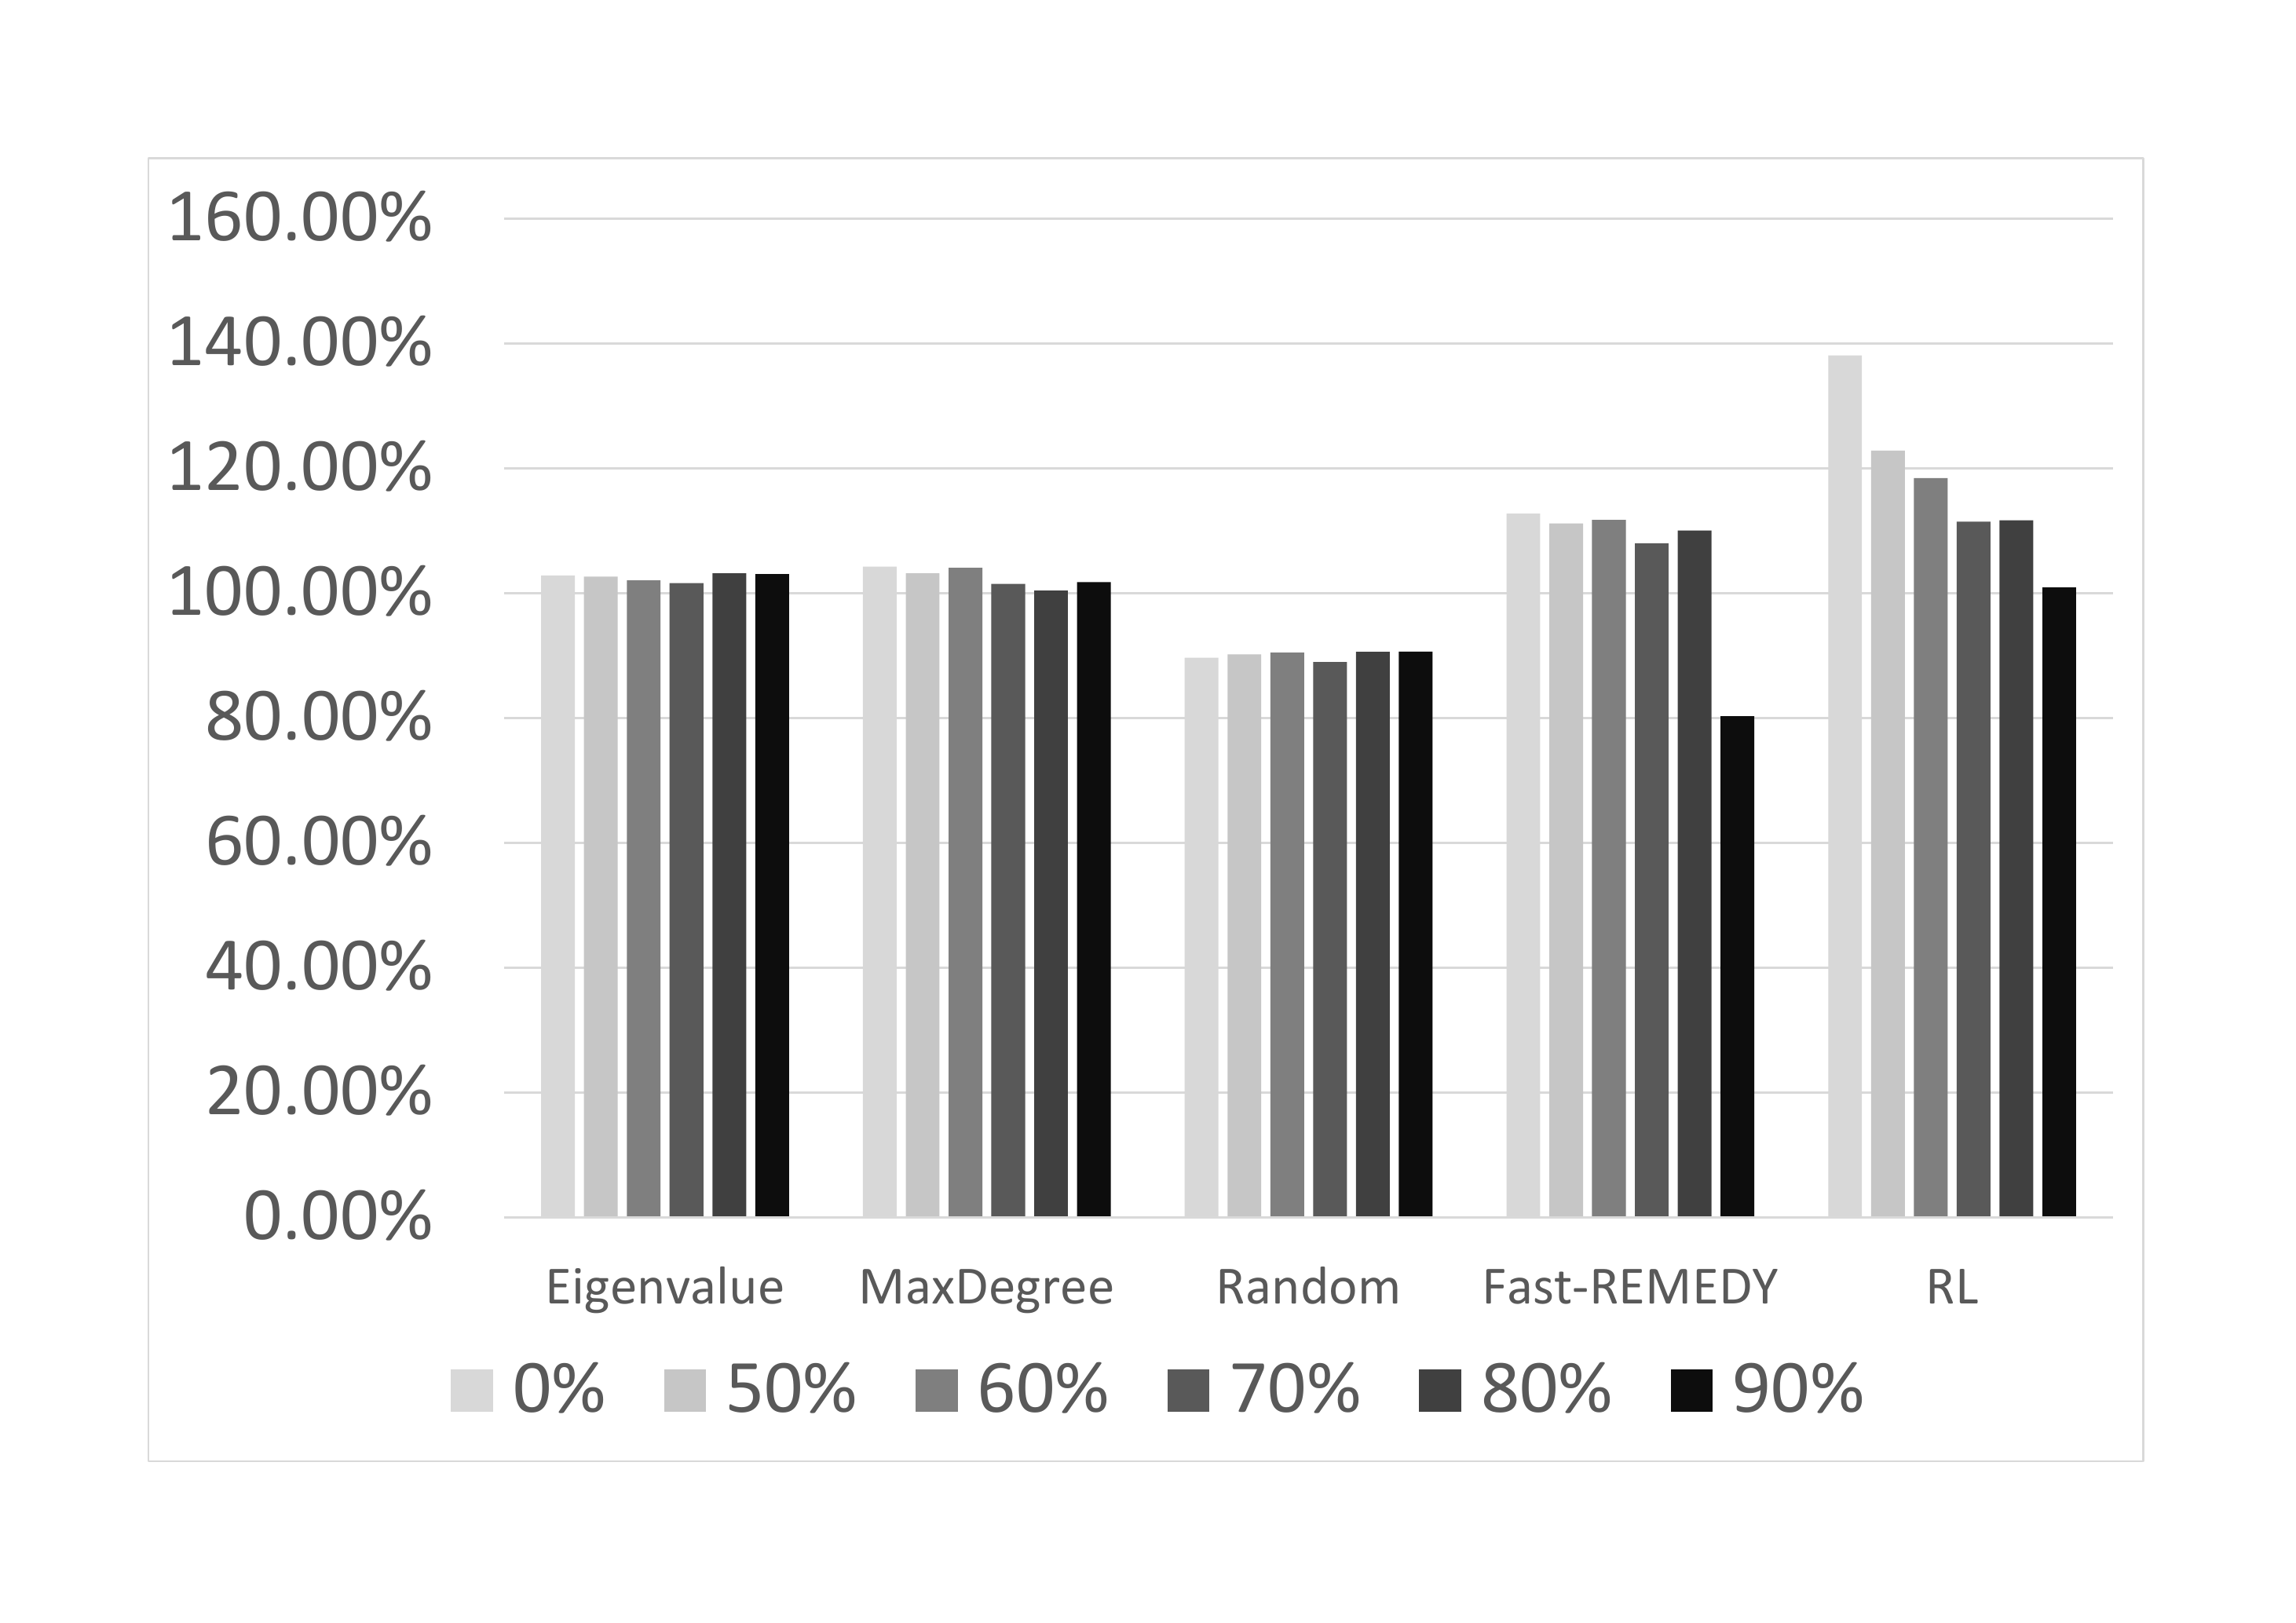}%
}\hfill
\centering
\caption{Performance under edge information removal.}\label{edge}
\end{figure*}

\begin{figure*}[t]
\centering
\subfloat[Hospital]{%
  \includegraphics[width=0.35\textwidth,keepaspectratio]{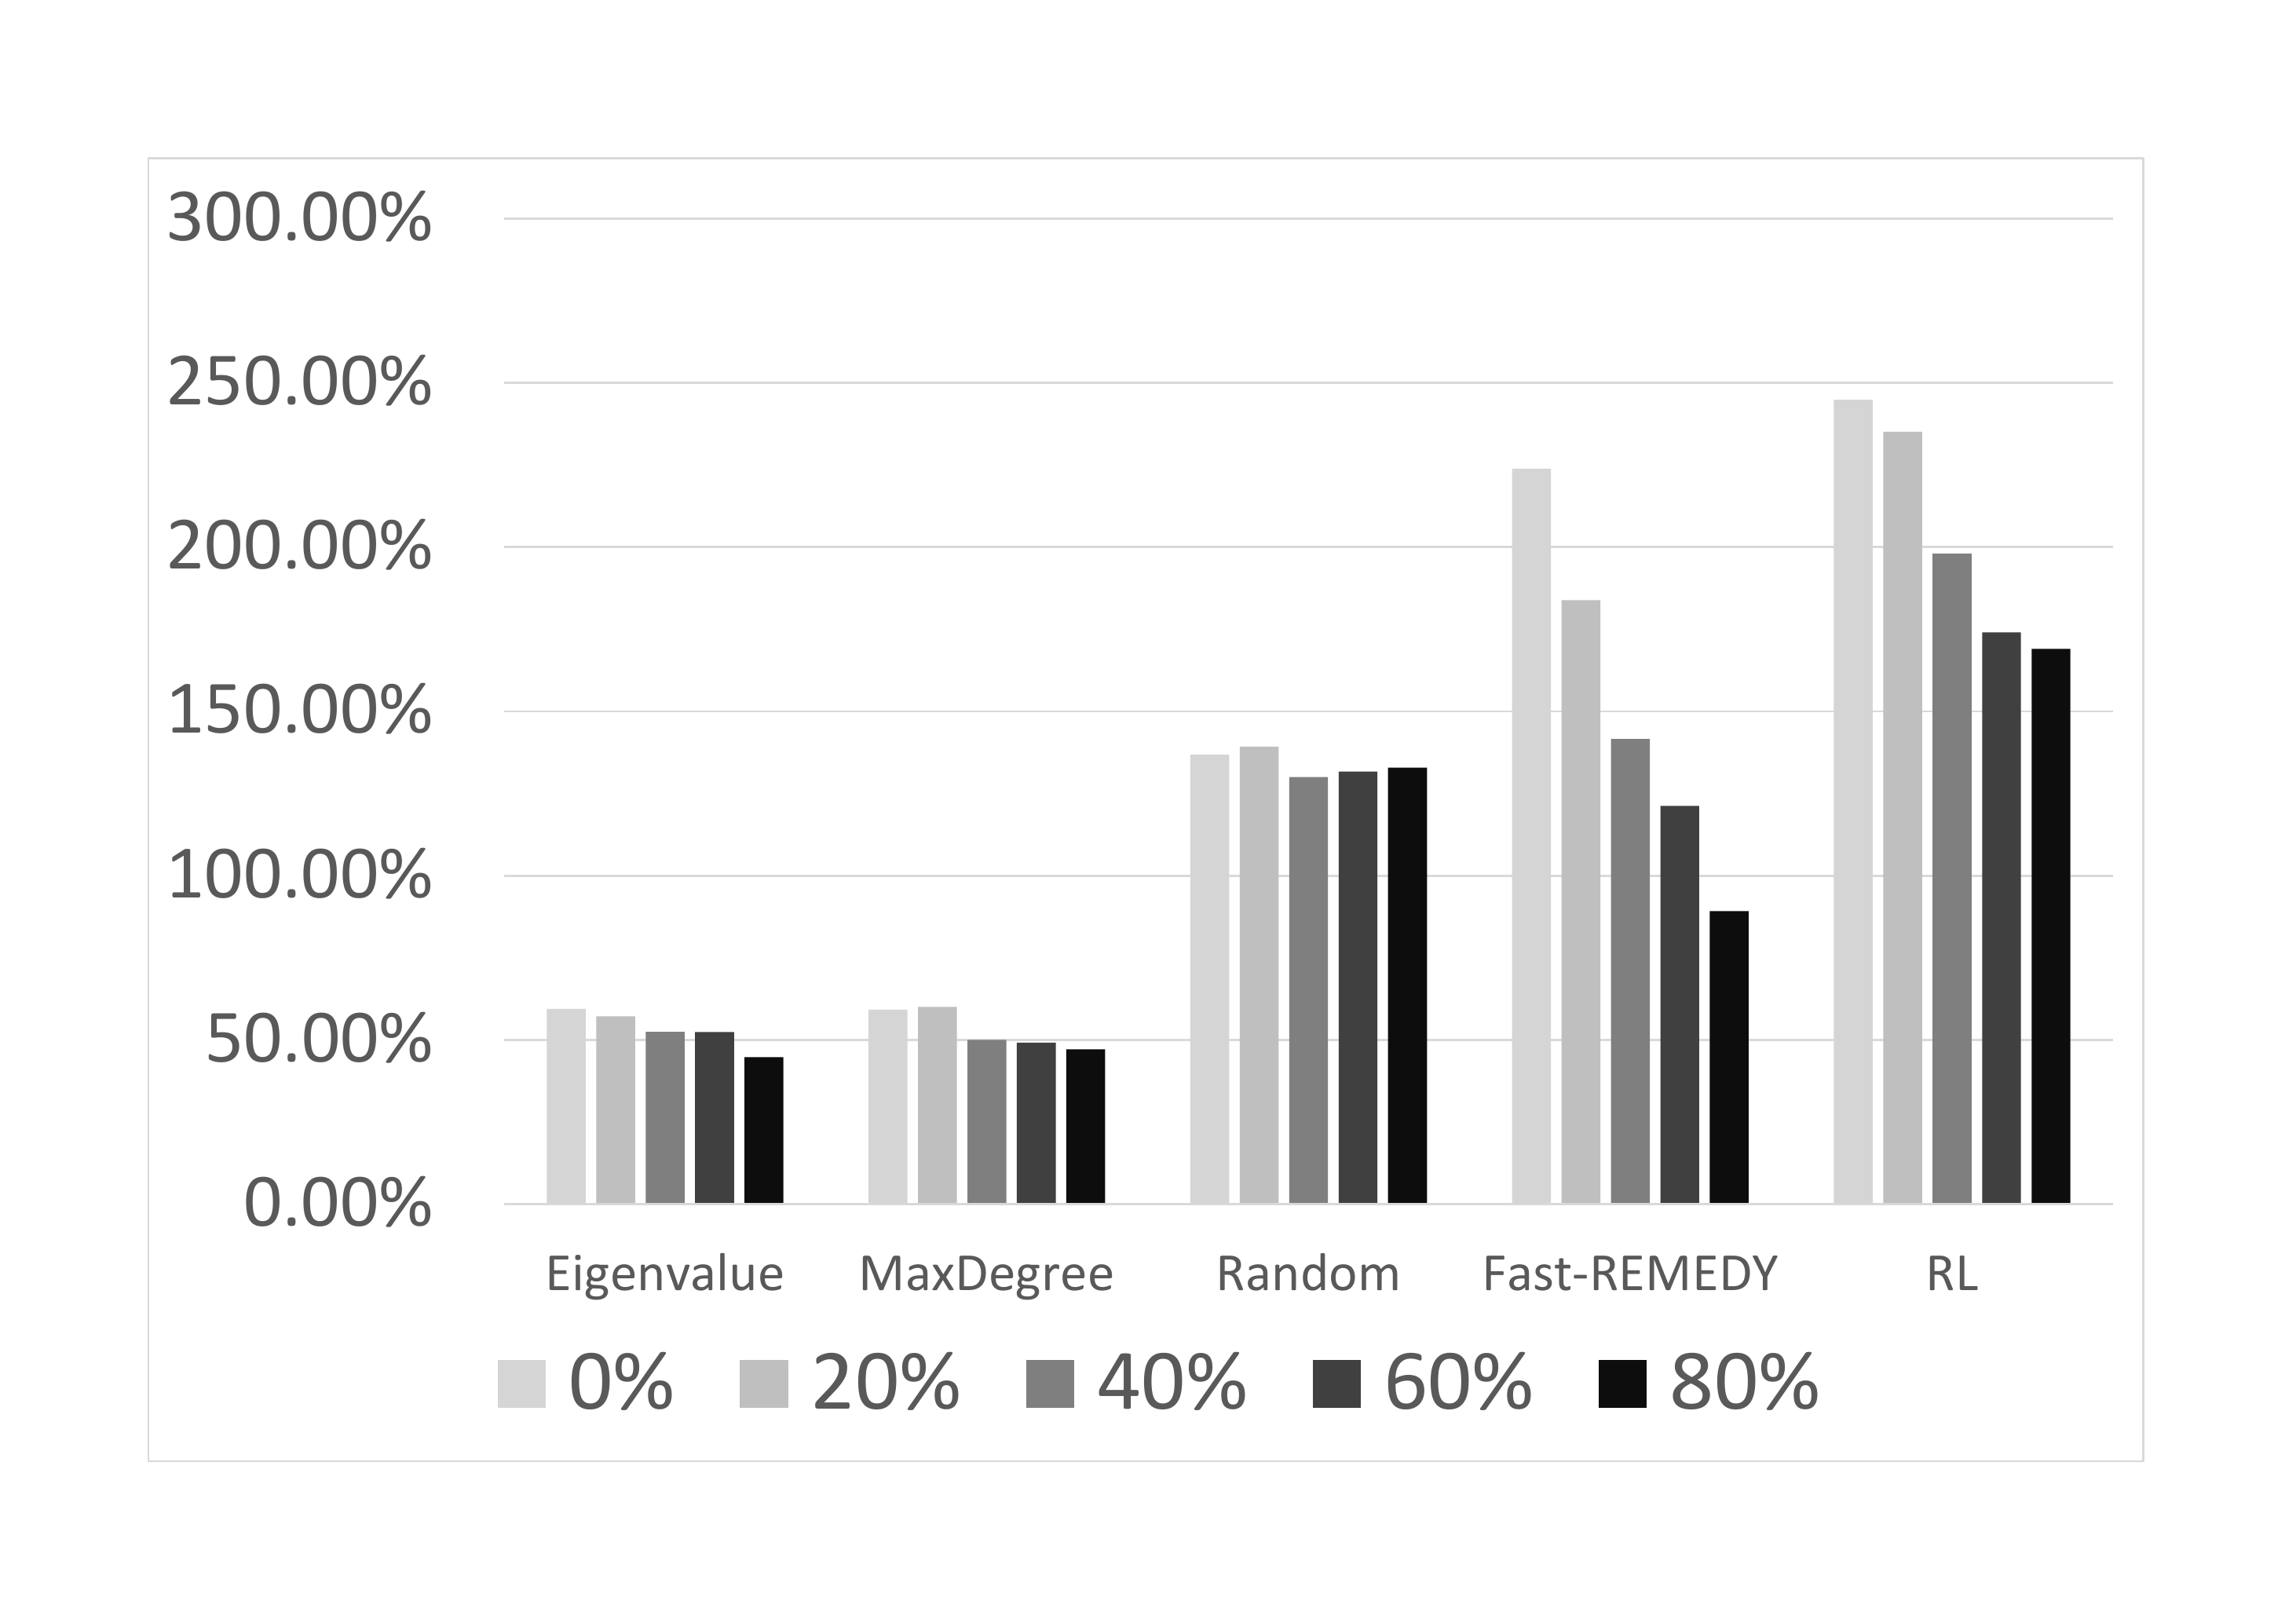}%
}\hfill
\subfloat[India]{%
  \includegraphics[width=0.35\textwidth,keepaspectratio]{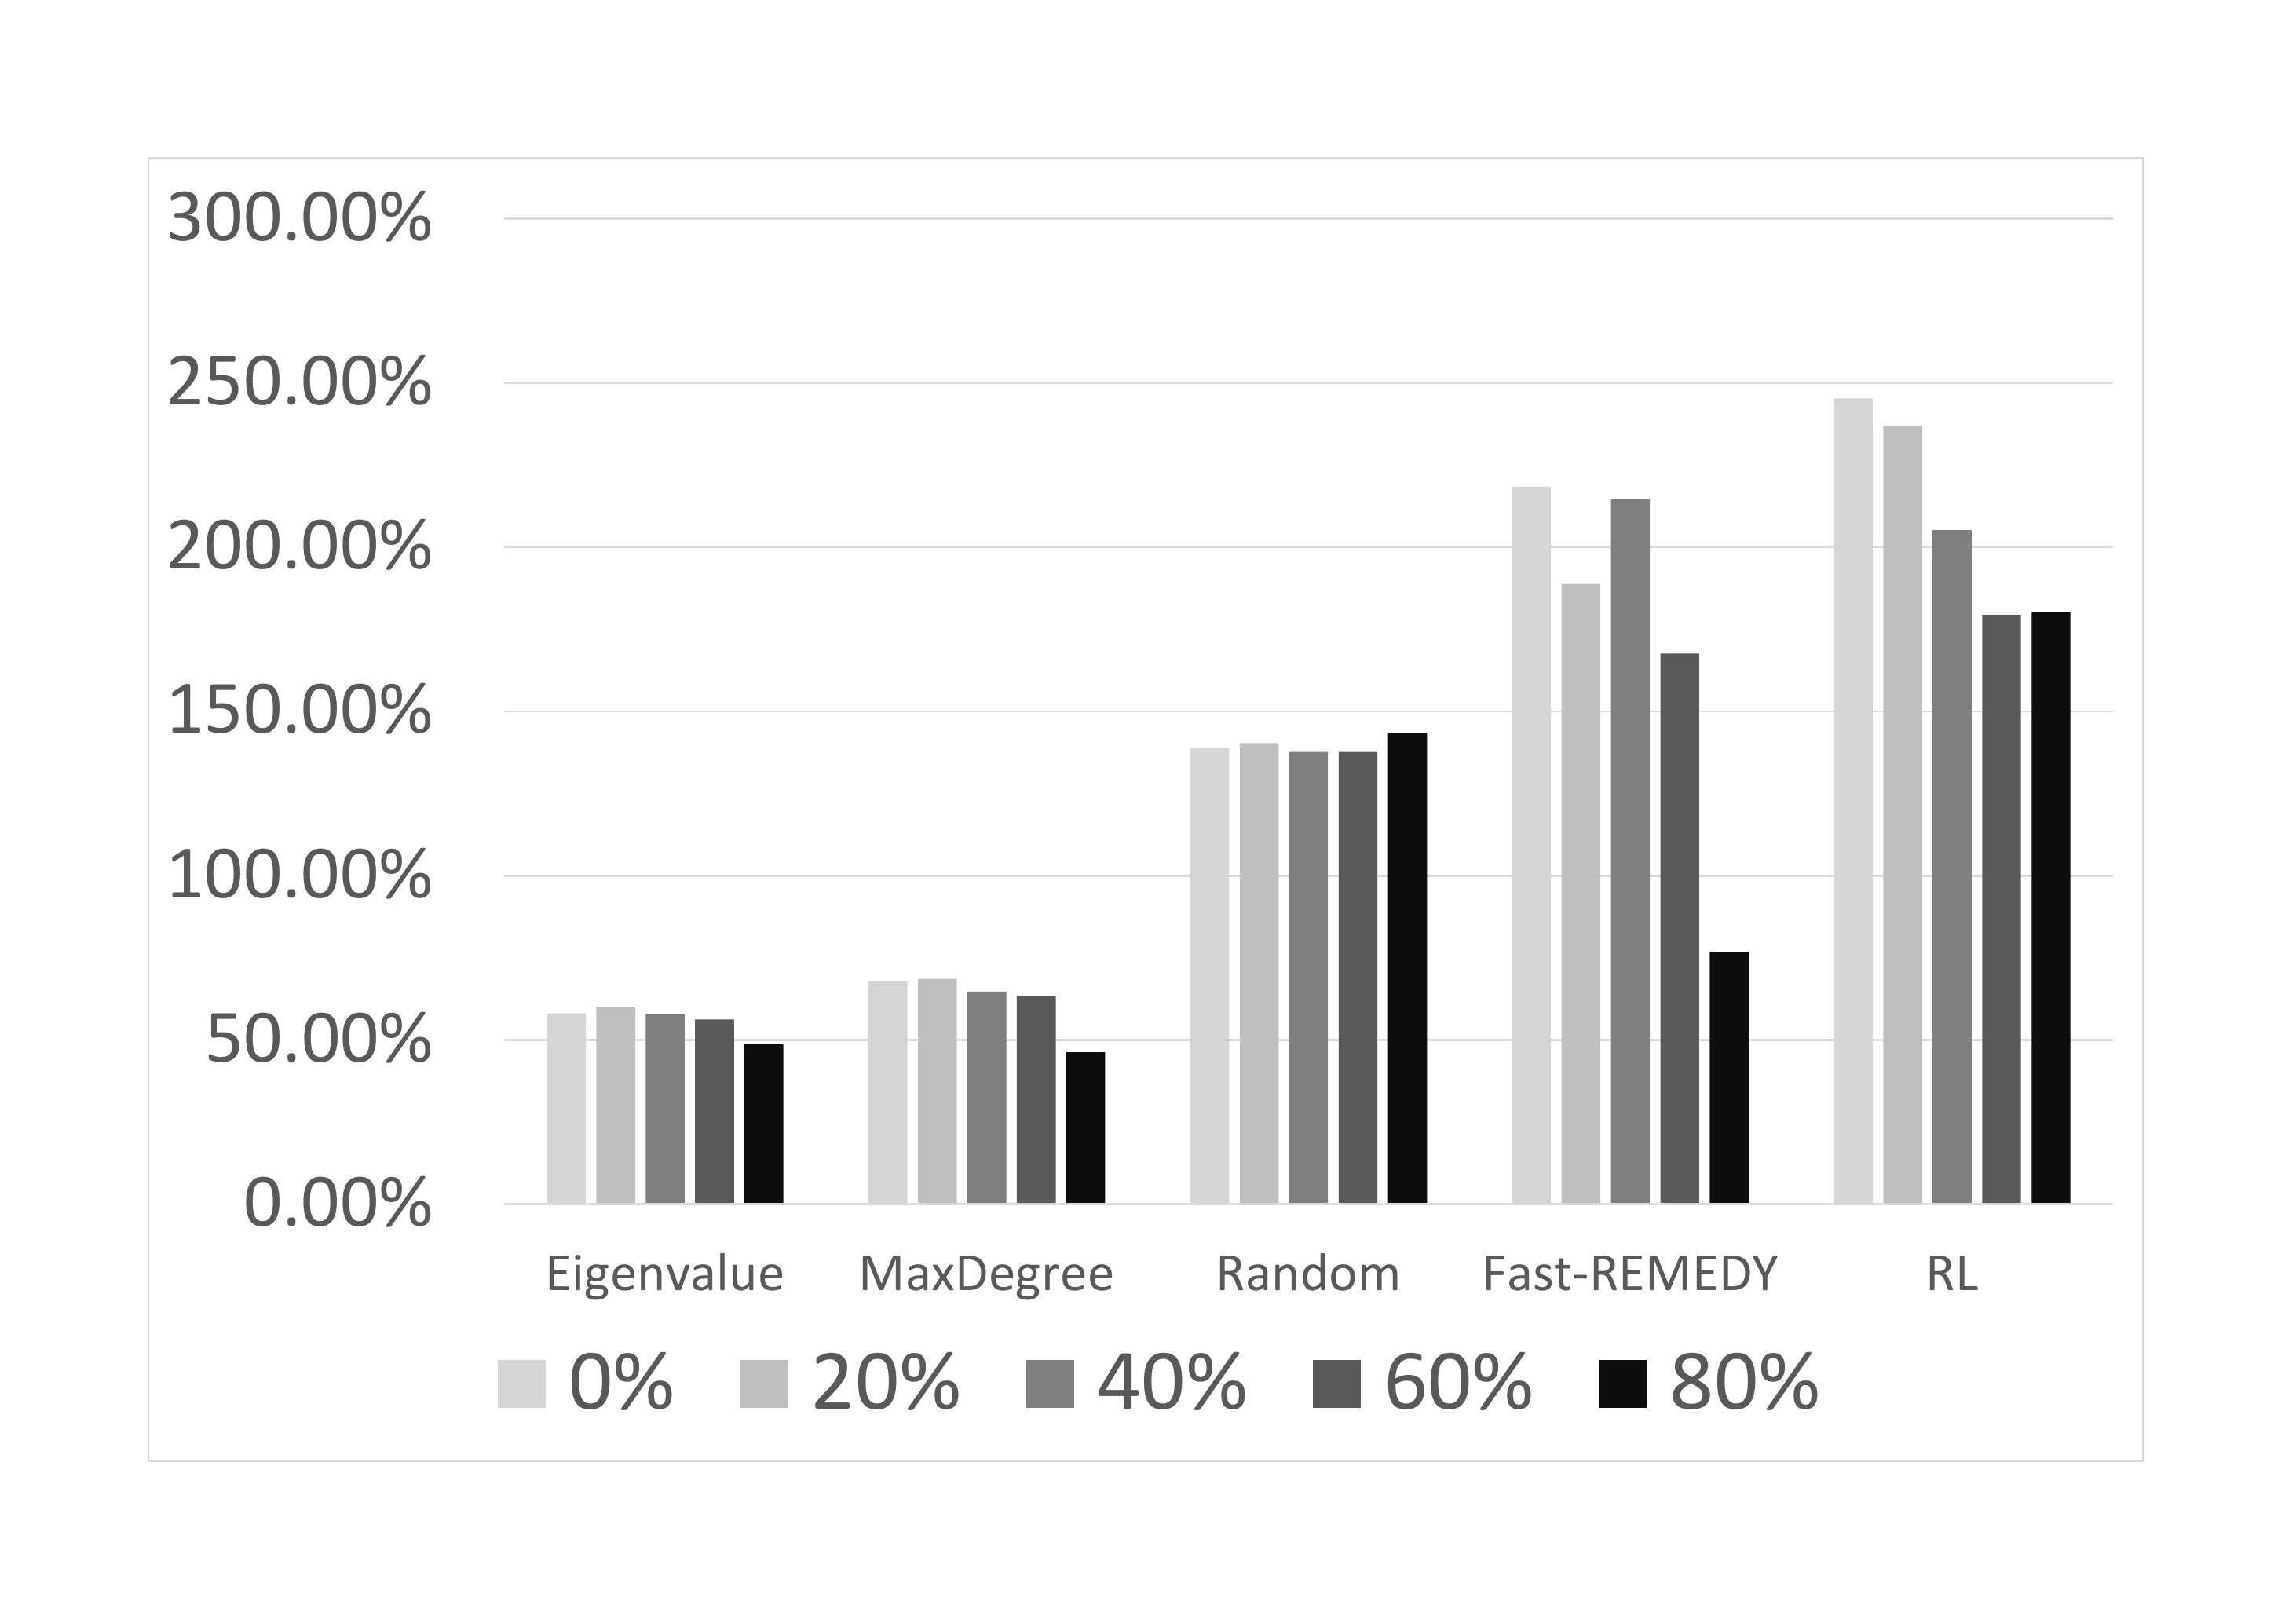}%
}\hfill
\subfloat[Flu]{%
  \includegraphics[width=0.35\textwidth,keepaspectratio]{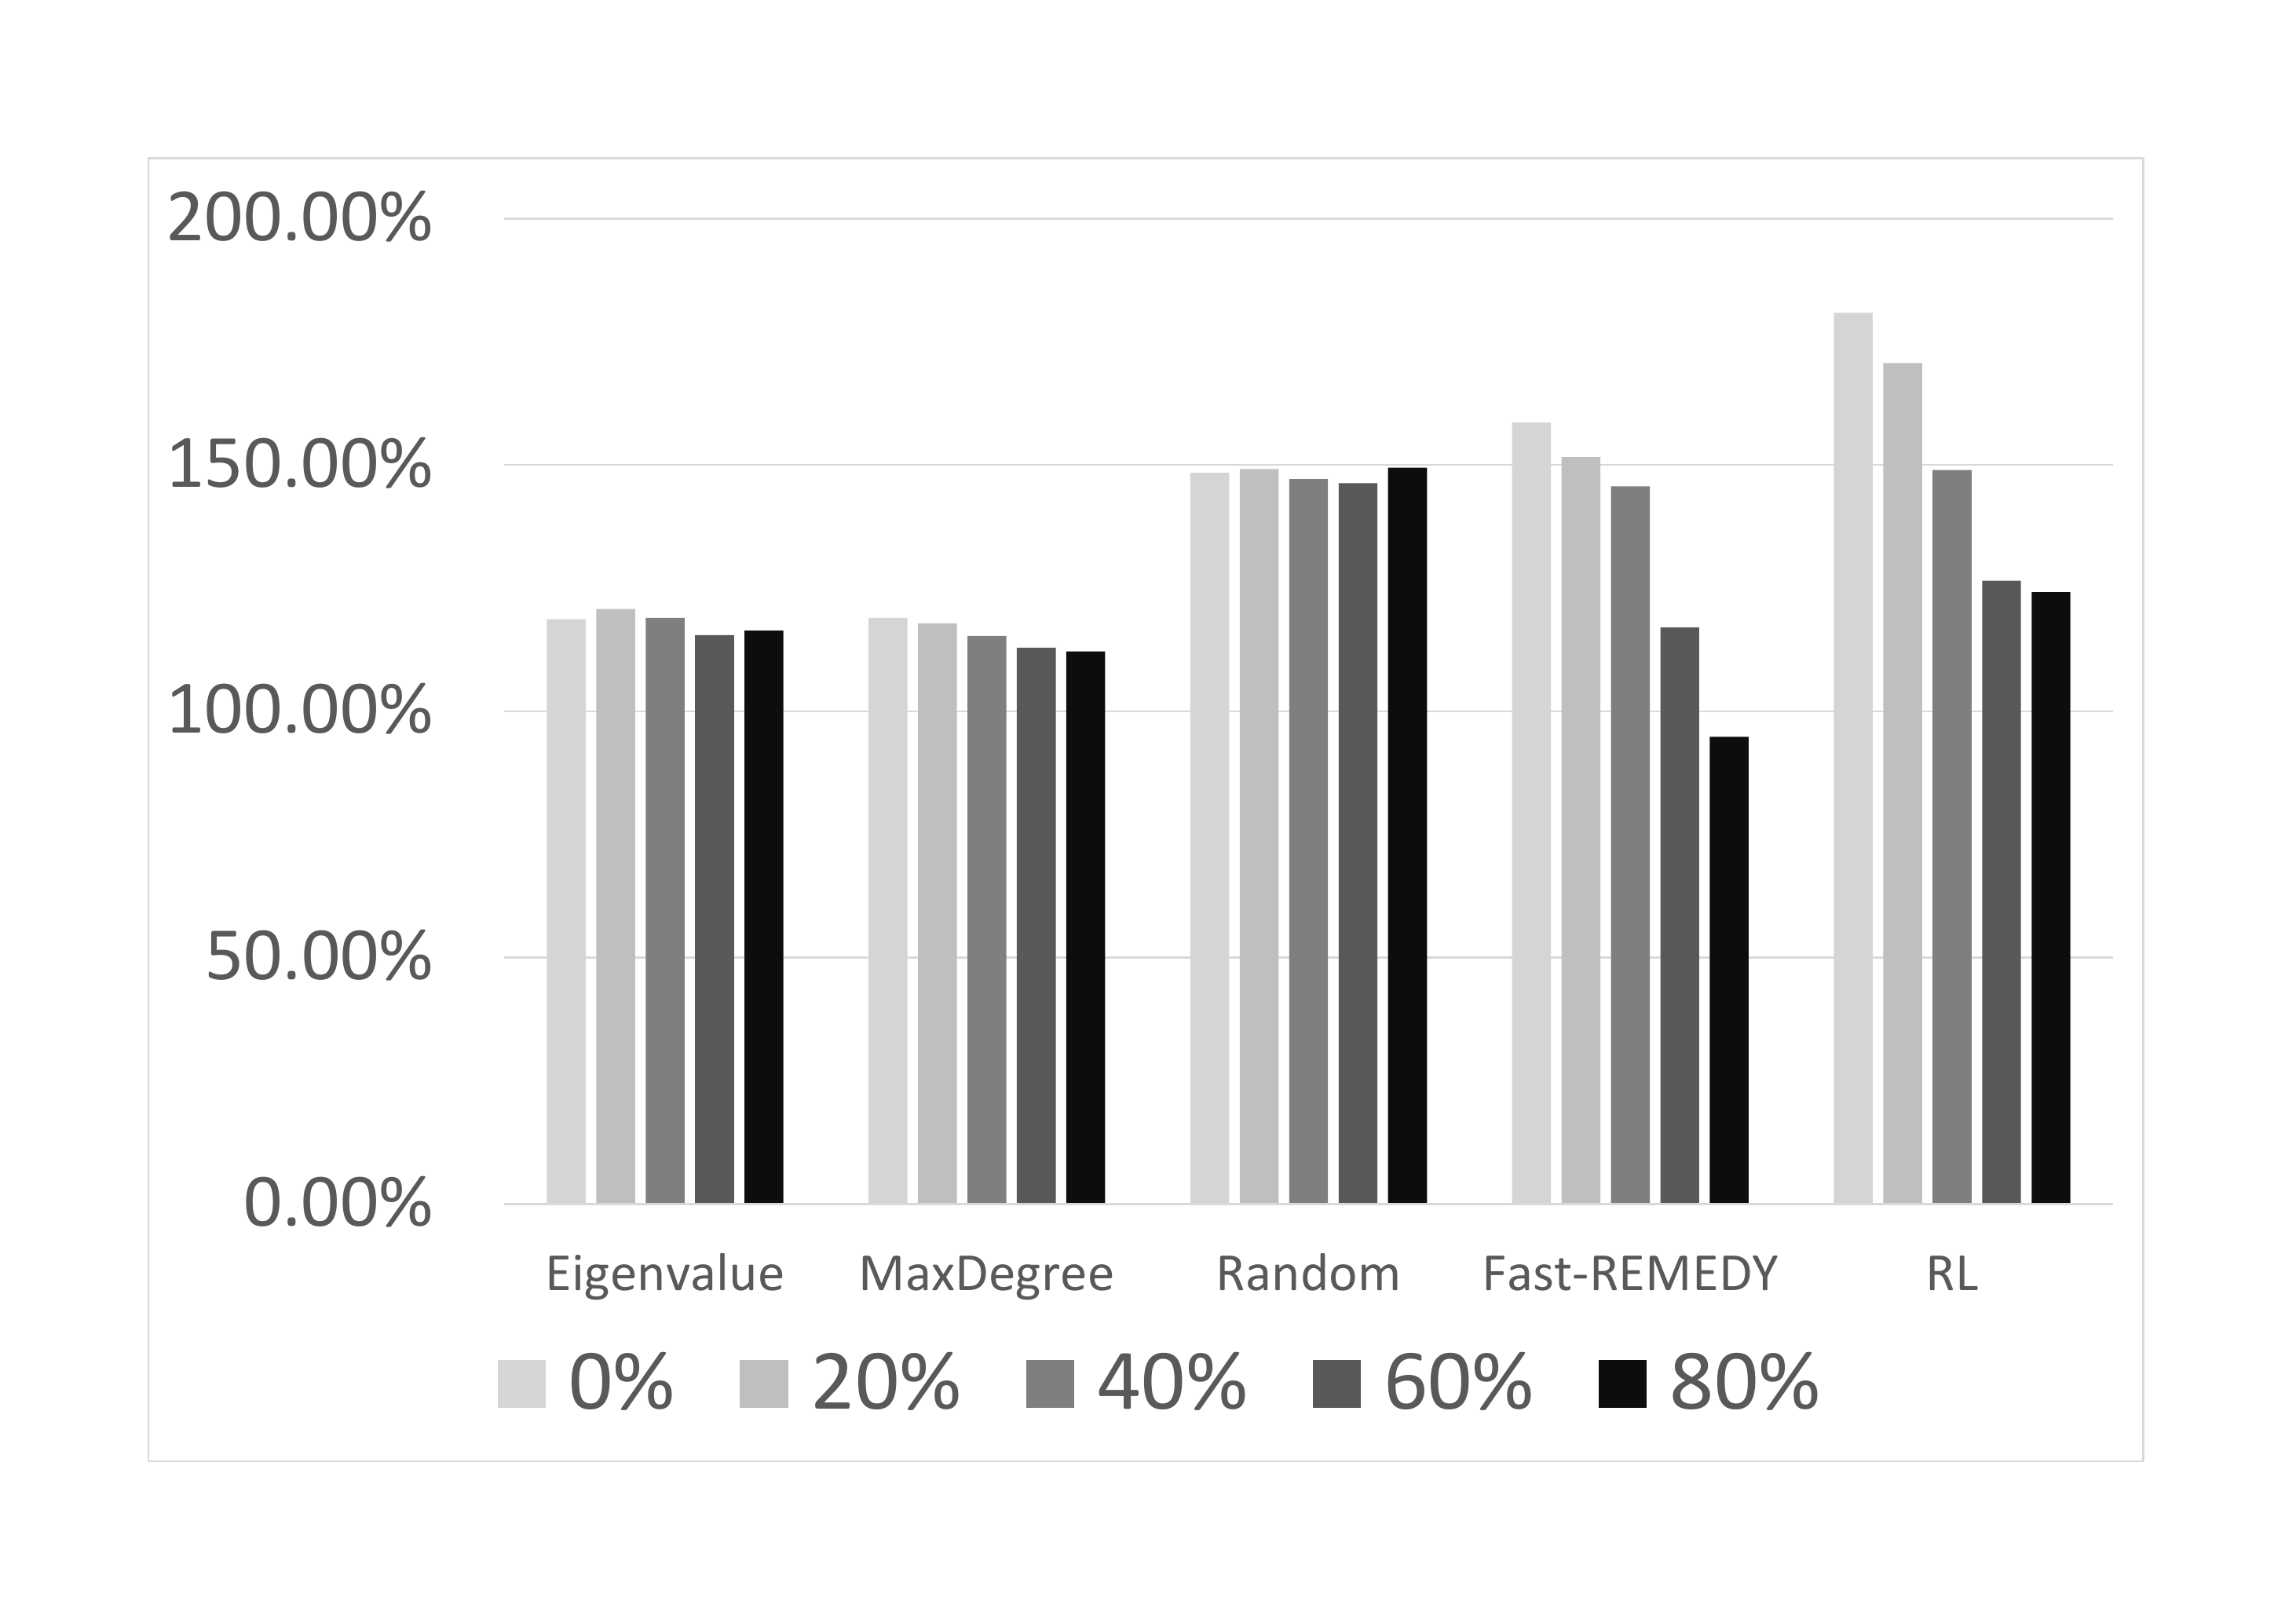}%
}\hfill
\subfloat[Irvine]{%
  \includegraphics[width=0.35\textwidth,keepaspectratio]{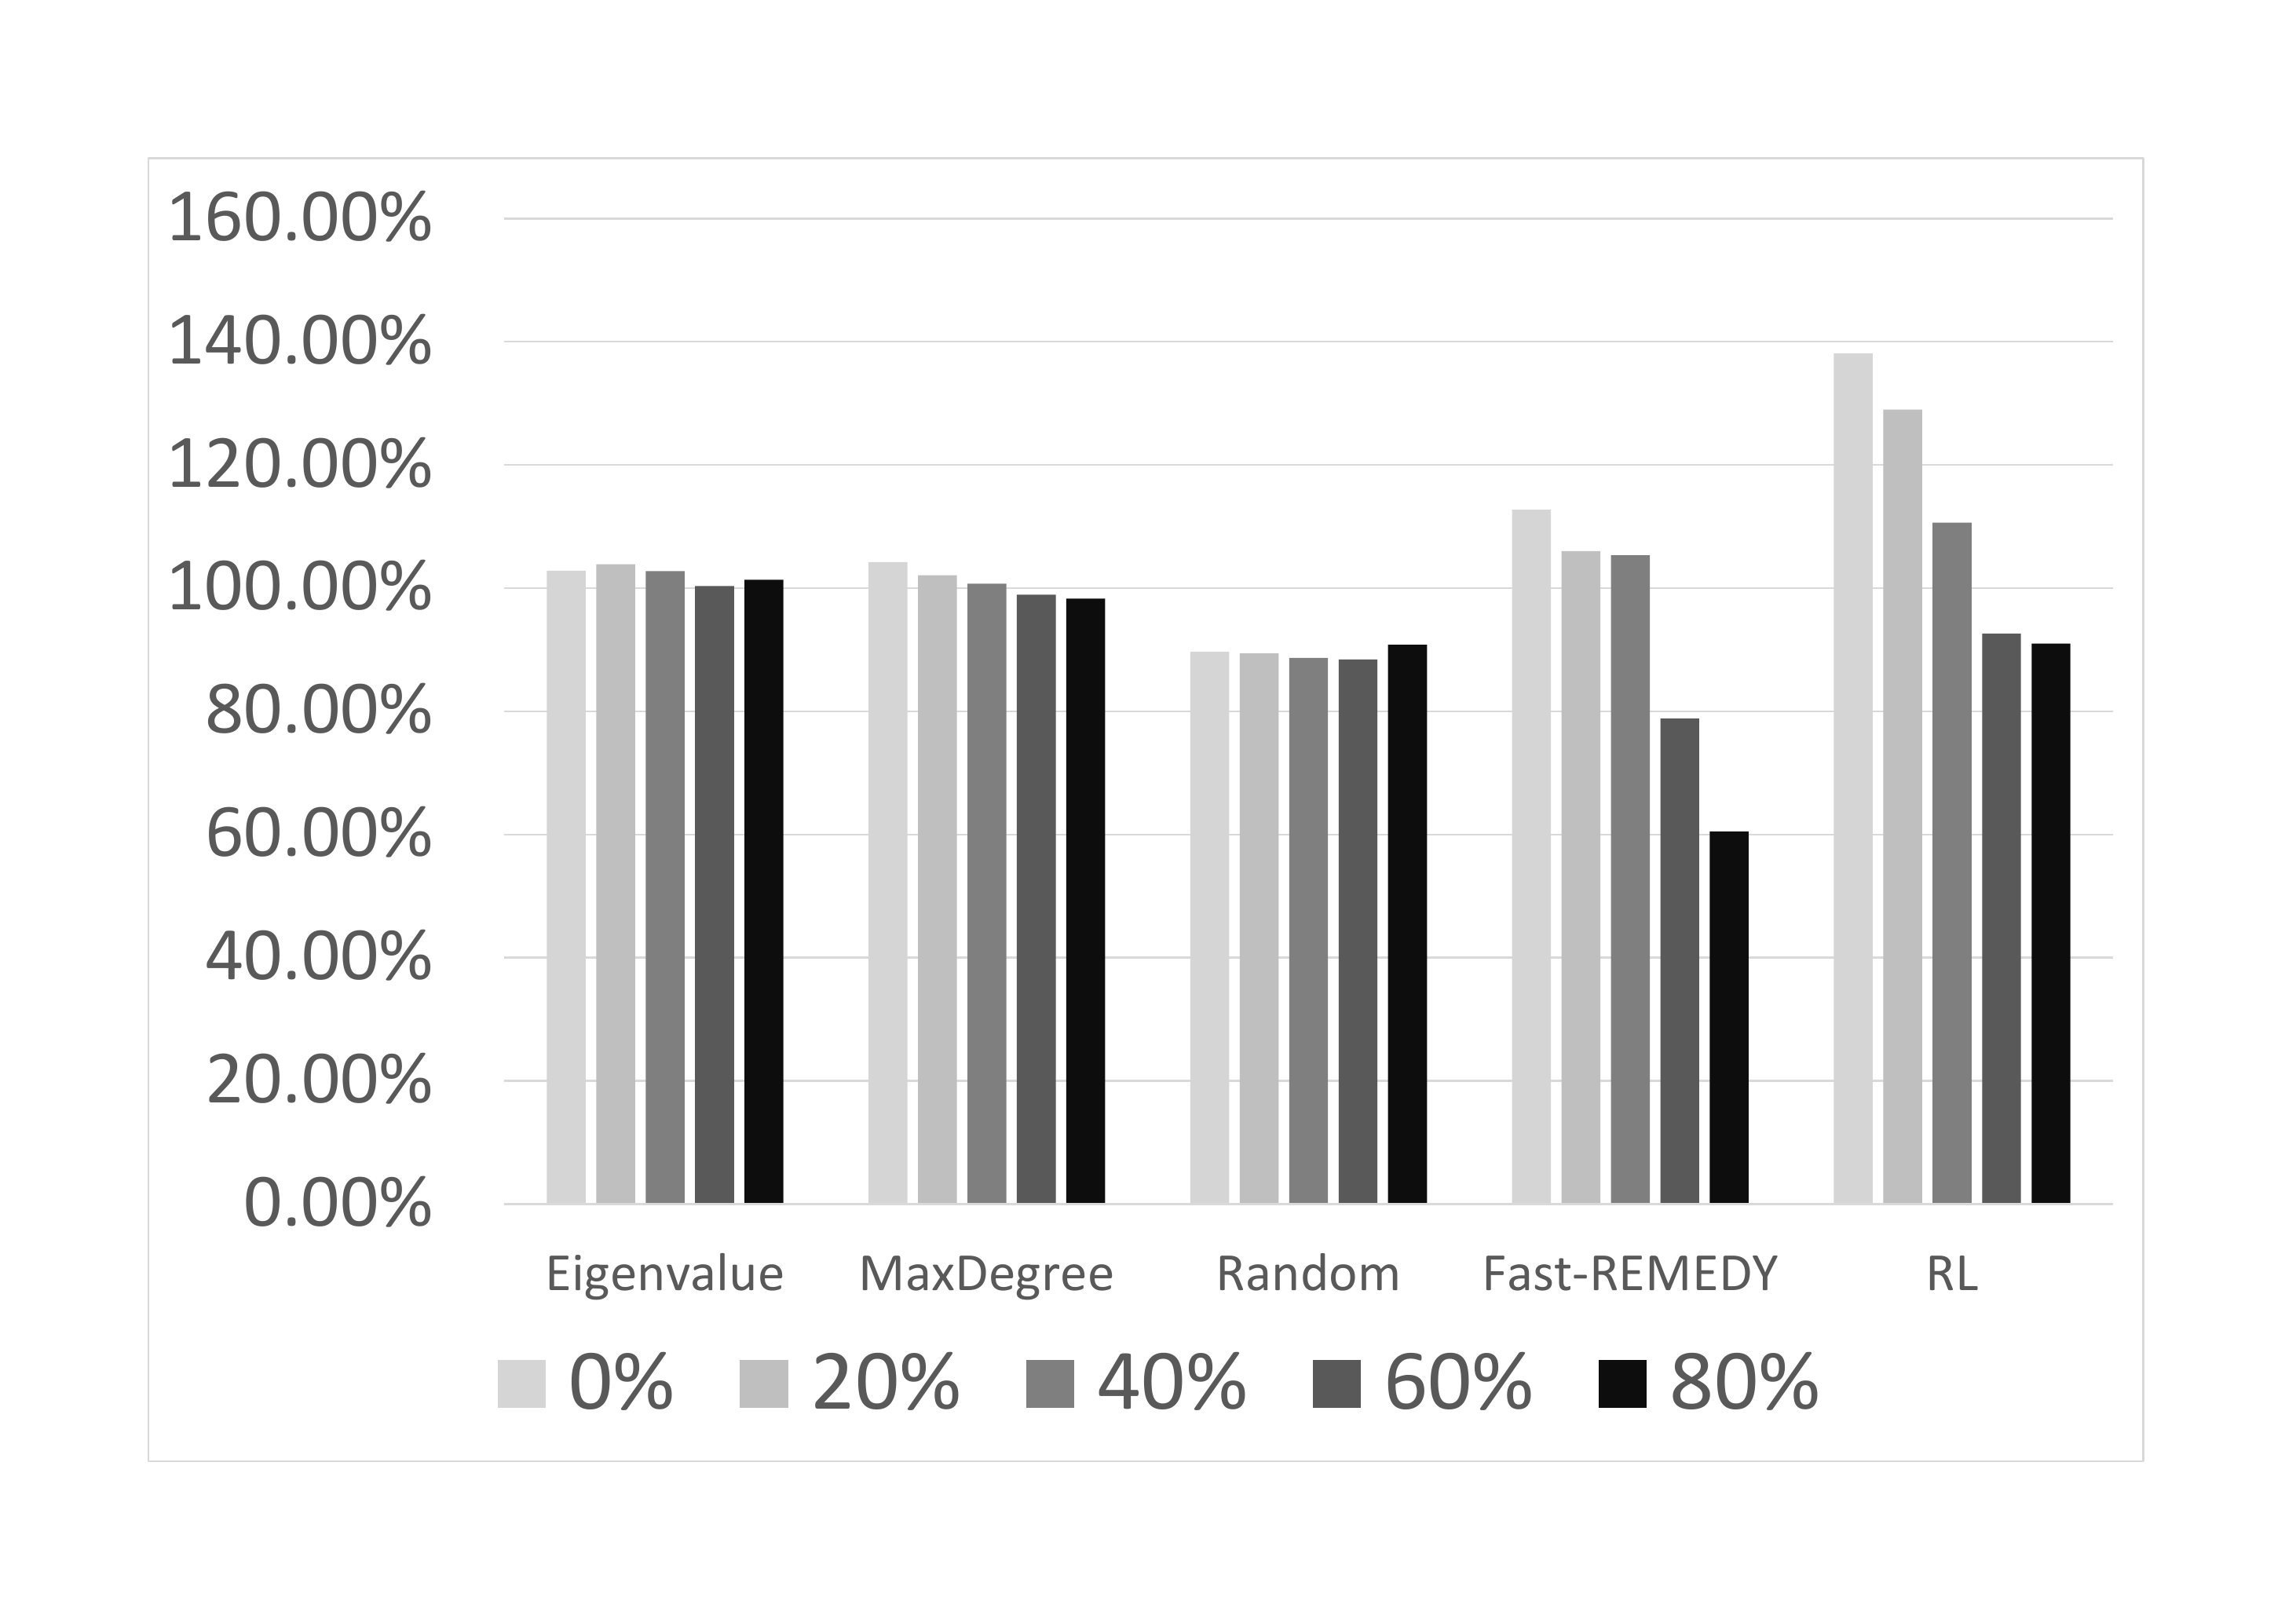}%
}\hfill
\centering
\caption{Performance under node information removal.}\label{node}
\end{figure*}
